# Supplementary material for: AI for trading strategies
Source: arXiv:2208.07168 source file (2022-06-26)
Supplement: Supplementary file 1 [file 7_Appendix.tex]

\section{Appendix}

\subsection{ARMA-GARCH Model}

The Augmented Dickey-Fuller test revealed no significant evidence of non-stationarity, with a p-value of 0 and a negative ADF-Statistic of -11.93. Now, let us have a look at the table \ref{ARMA: Des_stat}.

\begin{table}
\hfill
\begin{centering}
\caption{Descriptive statistics of Brent crude Oil closing Price }
\begin{tabular}{cccc}
\toprule[0.1pt]
\textbf{Statistic} & \textbf{Values}  \\\addlinespace
\midrule[0.1pt]\addlinespace
Mean & 77.384  \\\addlinespace
Median & 73.290  \\\addlinespace
Maximum & 146.080 \\\addlinespace
Minimum & 19.330 \\\addlinespace
Standard deviation & 25.870  \\\addlinespace
Skewness & 0.229  \\\addlinespace
Kurtosis & -1.029  \\\addlinespace
Jarque-Bera & 193.091 p-Val: 0.0 \\\addlinespace
Observations & 3653 \\\addlinespace
\bottomrule[0.1pt]\addlinespace[2pt]
\label{ARMA: Des_stat}
\end{tabular}\par
\end{centering}
\end{table}
\newpage

Based on the descriptive statistics, the assumption of a normal distribution can refute. The skewness of 0.229 indicates a right-skewed distribution. A further indication of no normal distribution is the negative kurtosis value of -1.029. The Jarque-Bera test confirms the assumption of no normal distribution. Since the p-value is 0, the null hypothesis that the distribution is normal can be rejected. Now let us have a look at the log returns. The QQ-Plot confirms the non-normality implied by the descriptive statistics. Fat tails can be seen at the right and left ends. This can also be seen when looking at the distribution of the Log Returns. However, the question arises of how the data is now distributed. We assume that the data follow a Students-t distribution, which the QQ-plot confirms. Nevertheless, outliers must be expected. This is shown in the figure \ref{ARMA-GARCH: Log Return Distribution and QQ-Plot's}.

\begin{figure}[h!]
  \centering
    \includegraphics[width=0.5\linewidth]{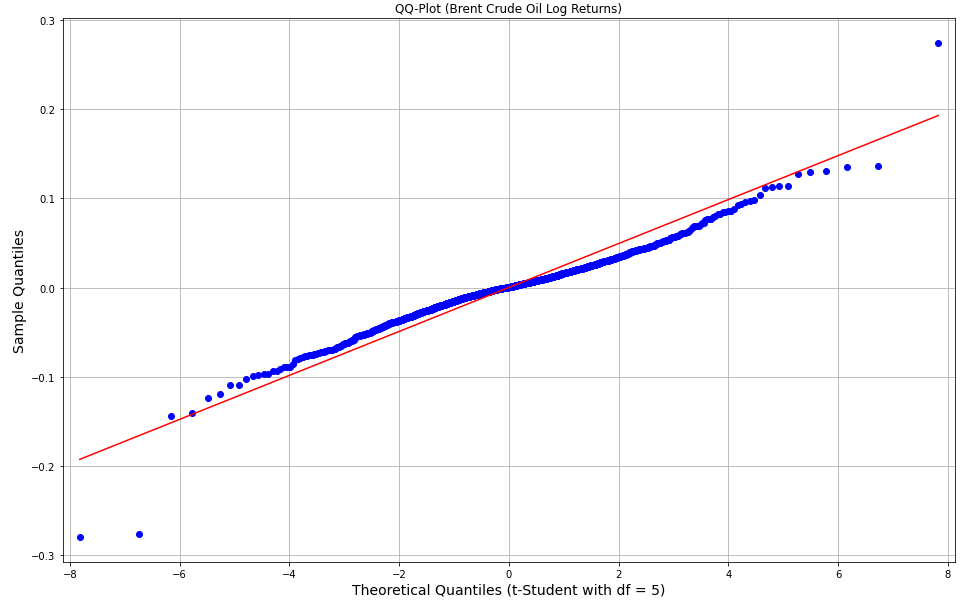}
    \includegraphics[width=0.5\linewidth]{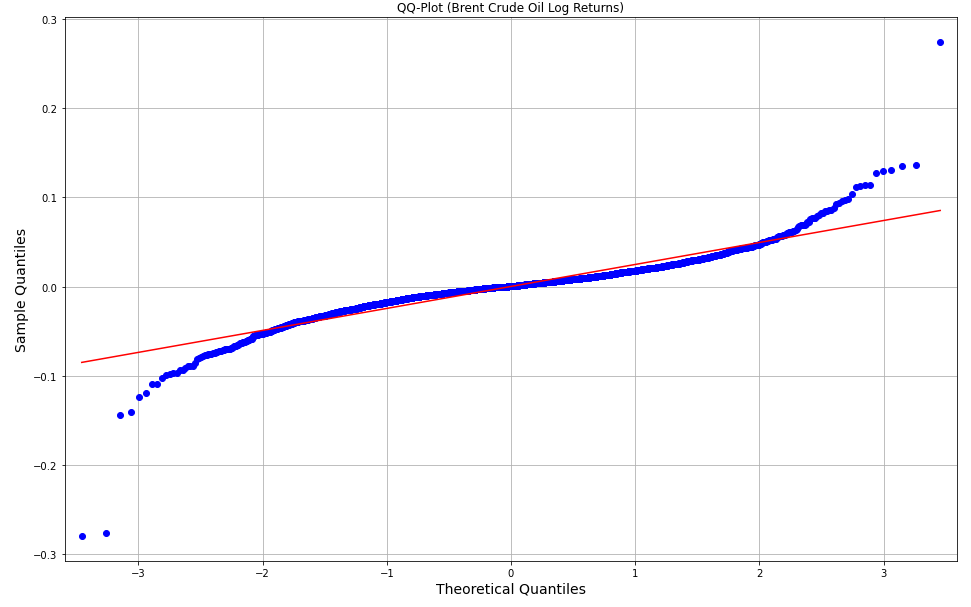}
    \includegraphics[width=0.5\linewidth]{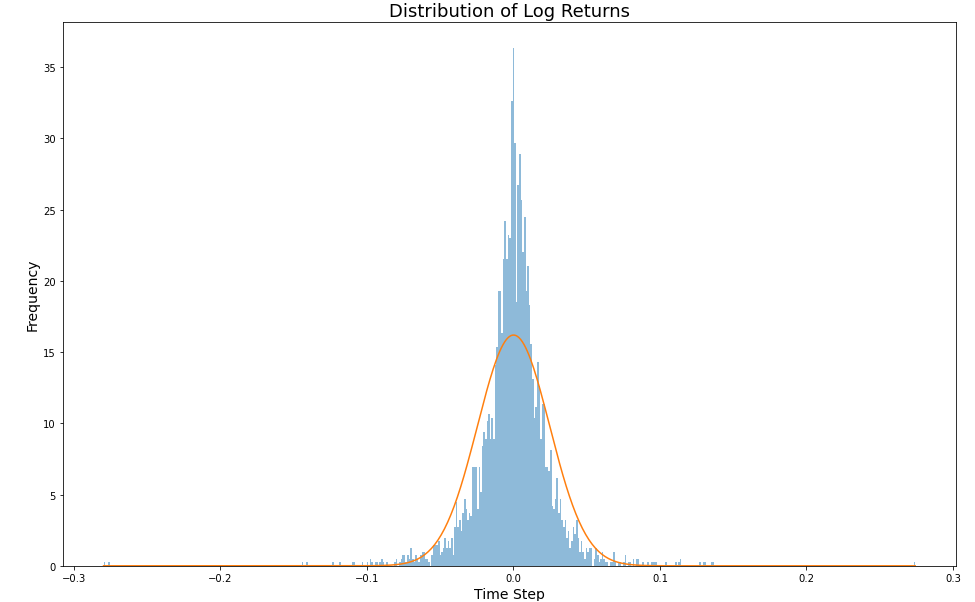}
    \caption{Log Return Distribution and QQ-Plot's}
    \label{ARMA-GARCH: Log Return Distribution and QQ-Plot's}
\end{figure}

\newpage
\textbf{Dependency structure}

Now the dependency structure is considered in more detail. The model order is determined with the help of the autocorrelation functions ACF and PACF. To examine this in more detail, one considers the following figure \ref{ARMA: QQ_plt} :

\begin{figure}[h!]
  \centering
    \includegraphics[width=0.5\linewidth]{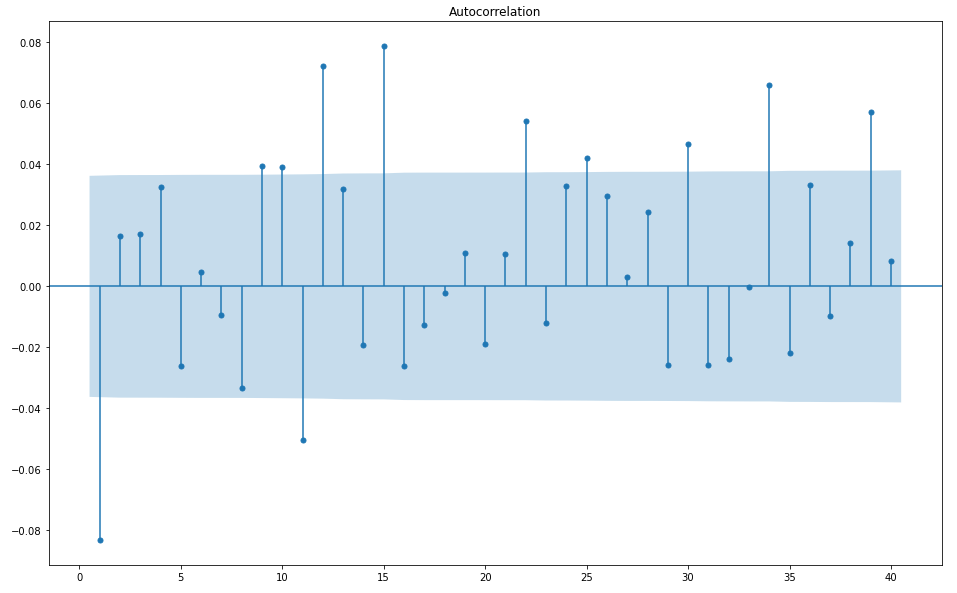}
    \includegraphics[width=0.5\linewidth]{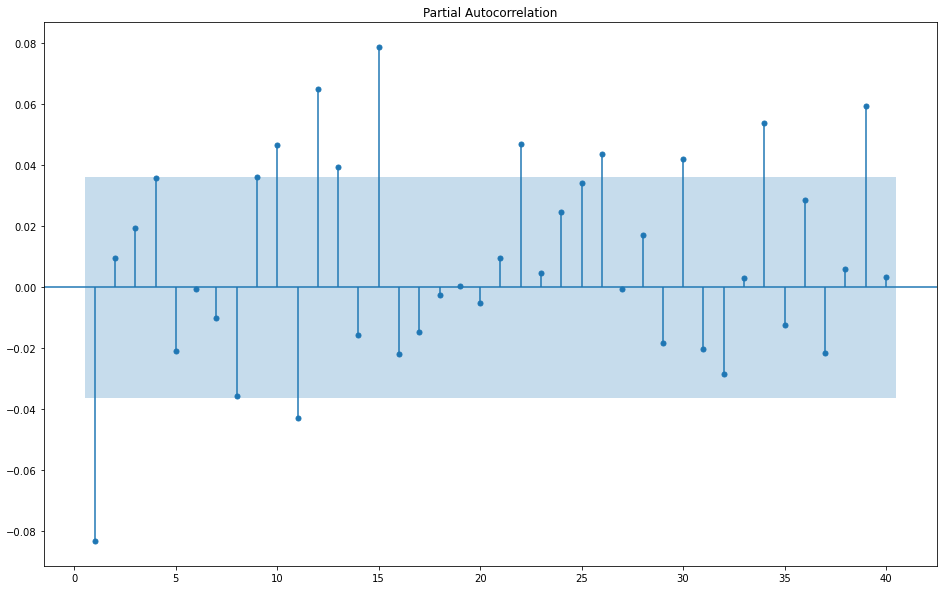}
    \caption{AFC and PACF}
    \label{ARMA: QQ_plt}
\end{figure}

The ACF shows dependence structures up to lag 49, but these are not considered because it is not assumed that data 49 days in the past have a significant influence on tomorrow's return. The same is also evident for the PACF at lag 44. Another reason for using minor possible model orders is model complexity. It was essential to keep the Model as simple as possible to explainable, and the result is not overfitted. Therefore, one assumes the model order ARMA(1,1). This will be examined in more detail in the next chapter using the Bayesian information criterion.

\newpage
\textbf{Building the ARMA(1,1)-GARCH(1,1) Model}

The ARMA(1,1)-GARCH(1,1) model is built in this section. GARCH processes are stationary (but not iid) white noise. In case the data is autocorrelated, the processes are misspecified. If this case happens, the pure ARMA and GARCH processes are defined as follows:
 
\begin{align}
\label{ARCH-GARCH Equations}
   y_{t} &= \mu + \sum_{i=1}^{p}a_{p}y_{t-p} + \epsilon_{t} + \sum_{i=1}^{q}b_{q}\epsilon_{t-q} \\
   \epsilon_{t} &= \sigma_{t}u_{t}\\
   \sigma{_t}^2 &= d + \sum_{i=1}^{n}\alpha_{n}\sigma_{t-n}^2+\sum_{i=1}^{m}\beta_{m}\epsilon_{t-m}^2
\end{align}

where $y_{t}$ describes the original data (typically non-stationary) and $\epsilon_{t}$ corresponds to the stationary log-return. This Model generalizes the ARMA family to the case of conditional heteroskedasticity (volatility clustering) and generalizes GARCH type models to processes with non-vanishing autocorrelation: $y_t$ is called the $ARMA(p,q)-GARCH(n,m)$-process. The identification of the model order now involves $p,q,m,n$. In many cases $n=m=1$ is used for financial data and in the case that $p,q \leq \ 1$, this serves as a good benchmark.

If one relies on the ACF/PACF analysis, one can see that residuals are significantly above the level at the lags 1, 4, 8, 10, and 15. One can use the BIC criteria to estimate the best possible Model Order. The ARMA(1,1) model has the lowest BIC of -14002. This confirms that we should use as simple an ARMA model as possible. To say something about the diagnostics of the Model, one can look at the Ljung box statistics in the table \ref{ARMA: Ljung-Box}. 

\begin{table}
\hfill
\begin{centering}
\caption{Ljung-Box Statitic of ARMA(1,1)-GARCH(1,1)}
\begin{tabular}{cccc}
\toprule[0.1pt]
\textbf{Lag}& \textbf{LB-Statistic} & \textbf{p-Value}\\\addlinespace
\midrule[0.1pt]\addlinespace
10 & 18.917444 & 4.132388e-02 \\\addlinespace
15 & 61.224745 & 1.551223e-07 \\\addlinespace
20  &  	64.187634 & 1.571243e-06\\\addlinespace
\bottomrule[0.1pt]\addlinespace[2pt]
\label{ARMA: Ljung-Box}
\end{tabular}\par
\end{centering}
\end{table}

The Ljung box Statistic looks good, as all p-values are below the 0.05 level. 

\newpage

\textbf{Parameter erstimation of ARMA(1,1)-GARCH(1,1)}

All estimated parameters are shown here (see table \ref{Parameter Estimatio ARMA}). 

\begin{table}
\hfill
\begin{centering}
\caption{Parameter Estimation of ARMA(1,1)-GARCH(1,1)}
\begin{tabular}{ccc}
\toprule[0.1pt]
\textbf{Parameter} & \textbf{ARMA(1,1)} & \textbf{GARCH(1,1)}\\\addlinespace
\midrule[0.1pt]\addlinespace
$a_1$  & -0.1805 & - \\\addlinespace
$\alpha_1$ & - & 0.0607 \\\addlinespace
$b_1$ & 0.993 &  -\\\addlinespace
$\beta_1$  &  -	 & 0.9386 \\\addlinespace
Log Likelihood  & 7020.987 	& -5868.3 \\\addlinespace
BIC  &  -14002.09 & 11776.5 \\\addlinespace
\bottomrule[0.1pt]\addlinespace[2pt]
\label{Parameter Estimatio ARMA}
\end{tabular}\par
\end{centering}
\end{table}

After modeling the ARMA(1,1) Model, the residuals are passed to the GARCH(1,1) model. Thus, the resulting conditional volatility can be calculated. This can be seen in the figure \ref{ARMA: Conditional Volatility}.

\begin{figure}[ht]
\begin{centering}
\includegraphics[width=10cm]{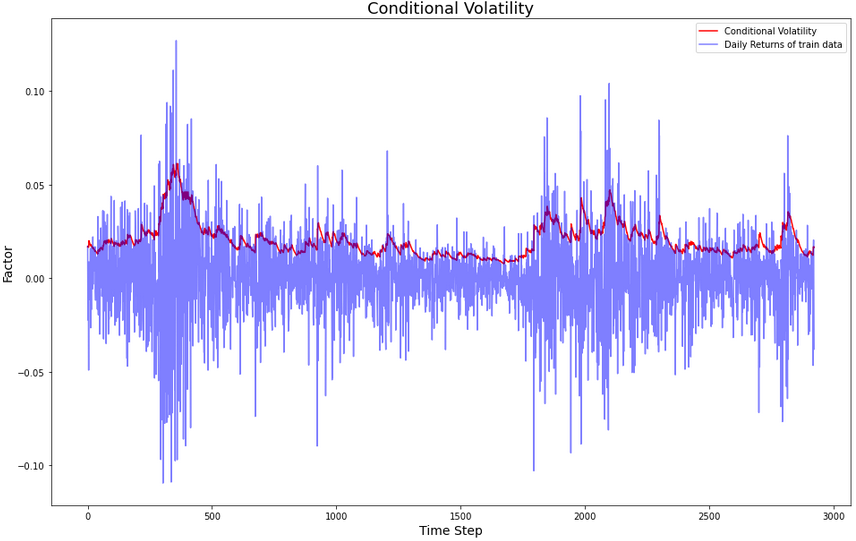}
\caption{Conditional Volatility}
\label{ARMA: Conditional Volatility}
\end{centering}
\end{figure}

\newpage

\textbf{ARMA-GARCH Model Prediction}

The prediction of the model can now be calculated using the formula \ref{ARCH-GARCH perd_equ}. 
\begin{equation}
\label{ARCH-GARCH perd_equ}
  y_{t}  = \mu + a_{1}y_{t-1} + \epsilon_{t} + b_{1}\epsilon_{t-1} 
\end{equation}

Figure \ref{ARMA-GARCH Prediciton} shows the test data with the predicted data.

\begin{figure}[ht]
\begin{centering}
\includegraphics[width=10cm]{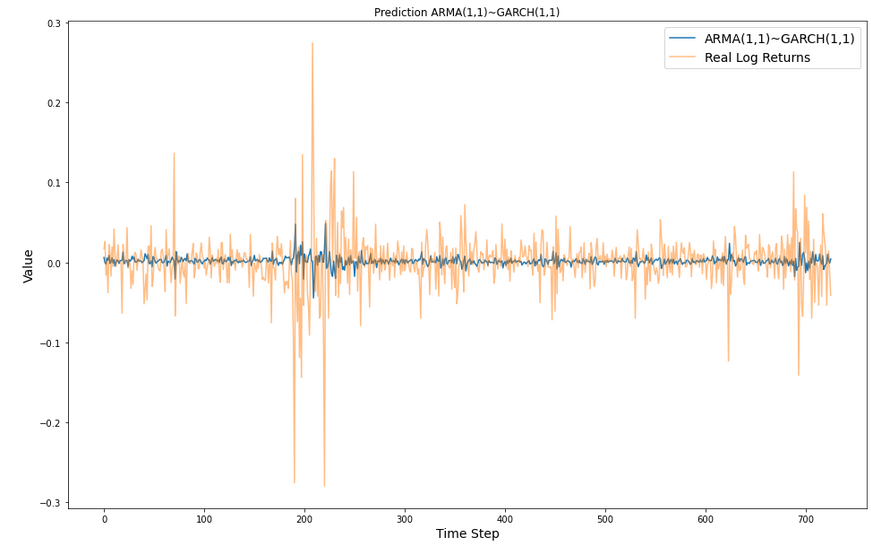}
\caption{ARMA-GARCH Prediciton}
\label{ARMA-GARCH Prediciton}
\end{centering}
\end{figure}

\newpage

\subsection{Classification Report}

To get a more detailed overview of how the models performed, one can build a classification report to compute the F1 Score, precision, recall, and support. The meaning of the variables can be interpreted as follows: 

\begin{align*}
\label{CR: Variable definition}
 t_{p} &= True Positiv \\
 f_{p} &= False Positiv \\
 f_{n} &= False Negativ 
\end{align*}

Precision measures the proportion of all correctly identified samples in a population of samples that are classified as positive labels and are defined as the following:

\begin{equation}
   \label{CR: Precision}
   \text{Precision} = \frac{t_{p}}{(t_{p}+f_{p})}
\end{equation}

The precision is intuitively the ability of the classifier not to label as positive a sample that is negative. The best value is 1, and the worst value is 0.

Recall (also known as sensitivity) measures the ability of a classifier to identify positive labels correctly and is defined as the following:

\begin{equation}
\label{CR: Recall2}
    Recall = \frac{t_{p}}{(t_{p}+f_{n})}
\end{equation}

The recall is intuitively the ability of the classifier to find all the positive samples. The best value is 1, and the worst value is 0.

Support is the number of actual occurrences of the class in the specified data-set. Imbalanced support in the training data may indicate structural weaknesses in the reported scores of the classifier and could indicate the need for stratified sampling or re-balancing. Support does not change between models but instead diagnoses the evaluation process. In some cases, we will have models that may have low precision or high recall. It is difficult to compare two models with low precision and high recall or vice versa. To make results comparable, we use a metric called the F-Score. The F-score helps to measure Recall and Precision at the same time. It uses Harmonic Mean in place of Arithmetic Mean by punishing the extreme values more. The traditional F-measure or balanced F-score (F1 score) is the harmonic mean of precision and recall:

\begin{equation}
\label{CR: F1-score}
    F1 Score = \frac{t_{p}}{(t_{p}+ \frac{1}{2}(f_{p}+f_{n}))}
\end{equation}

\subsection{Python Codes}
\includepdf[pages=-]{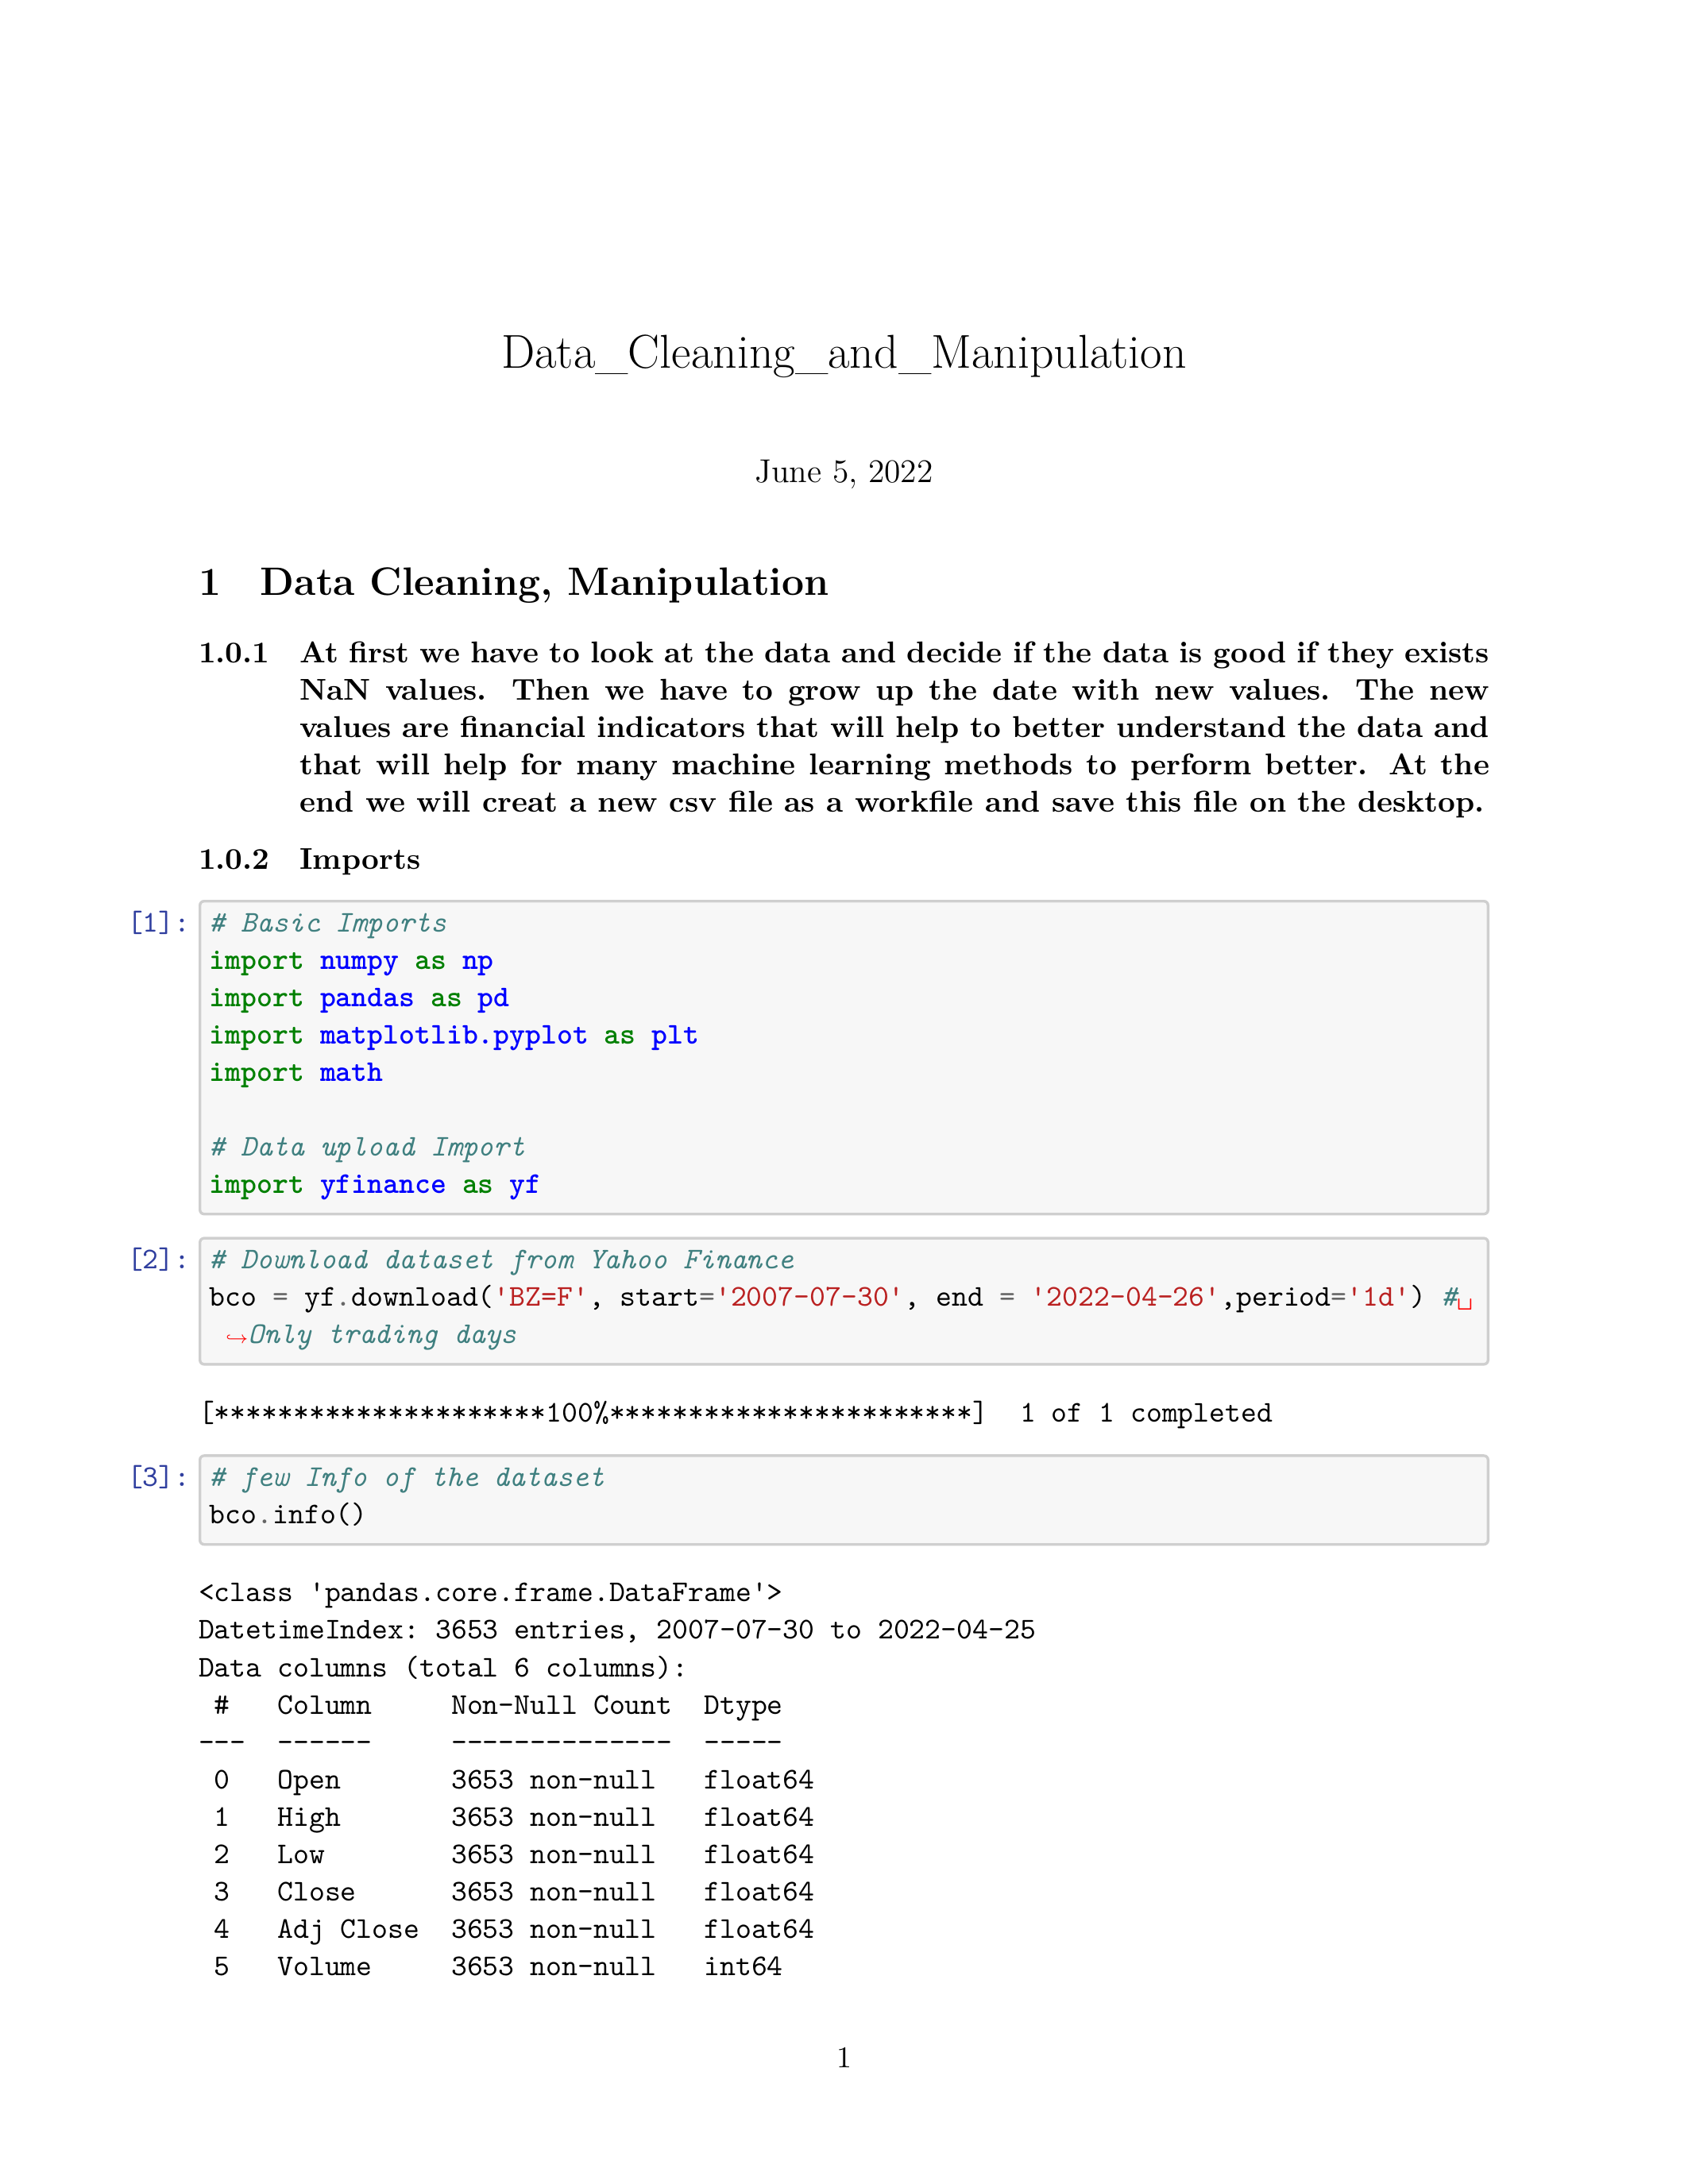}
\includepdf[pages=-]{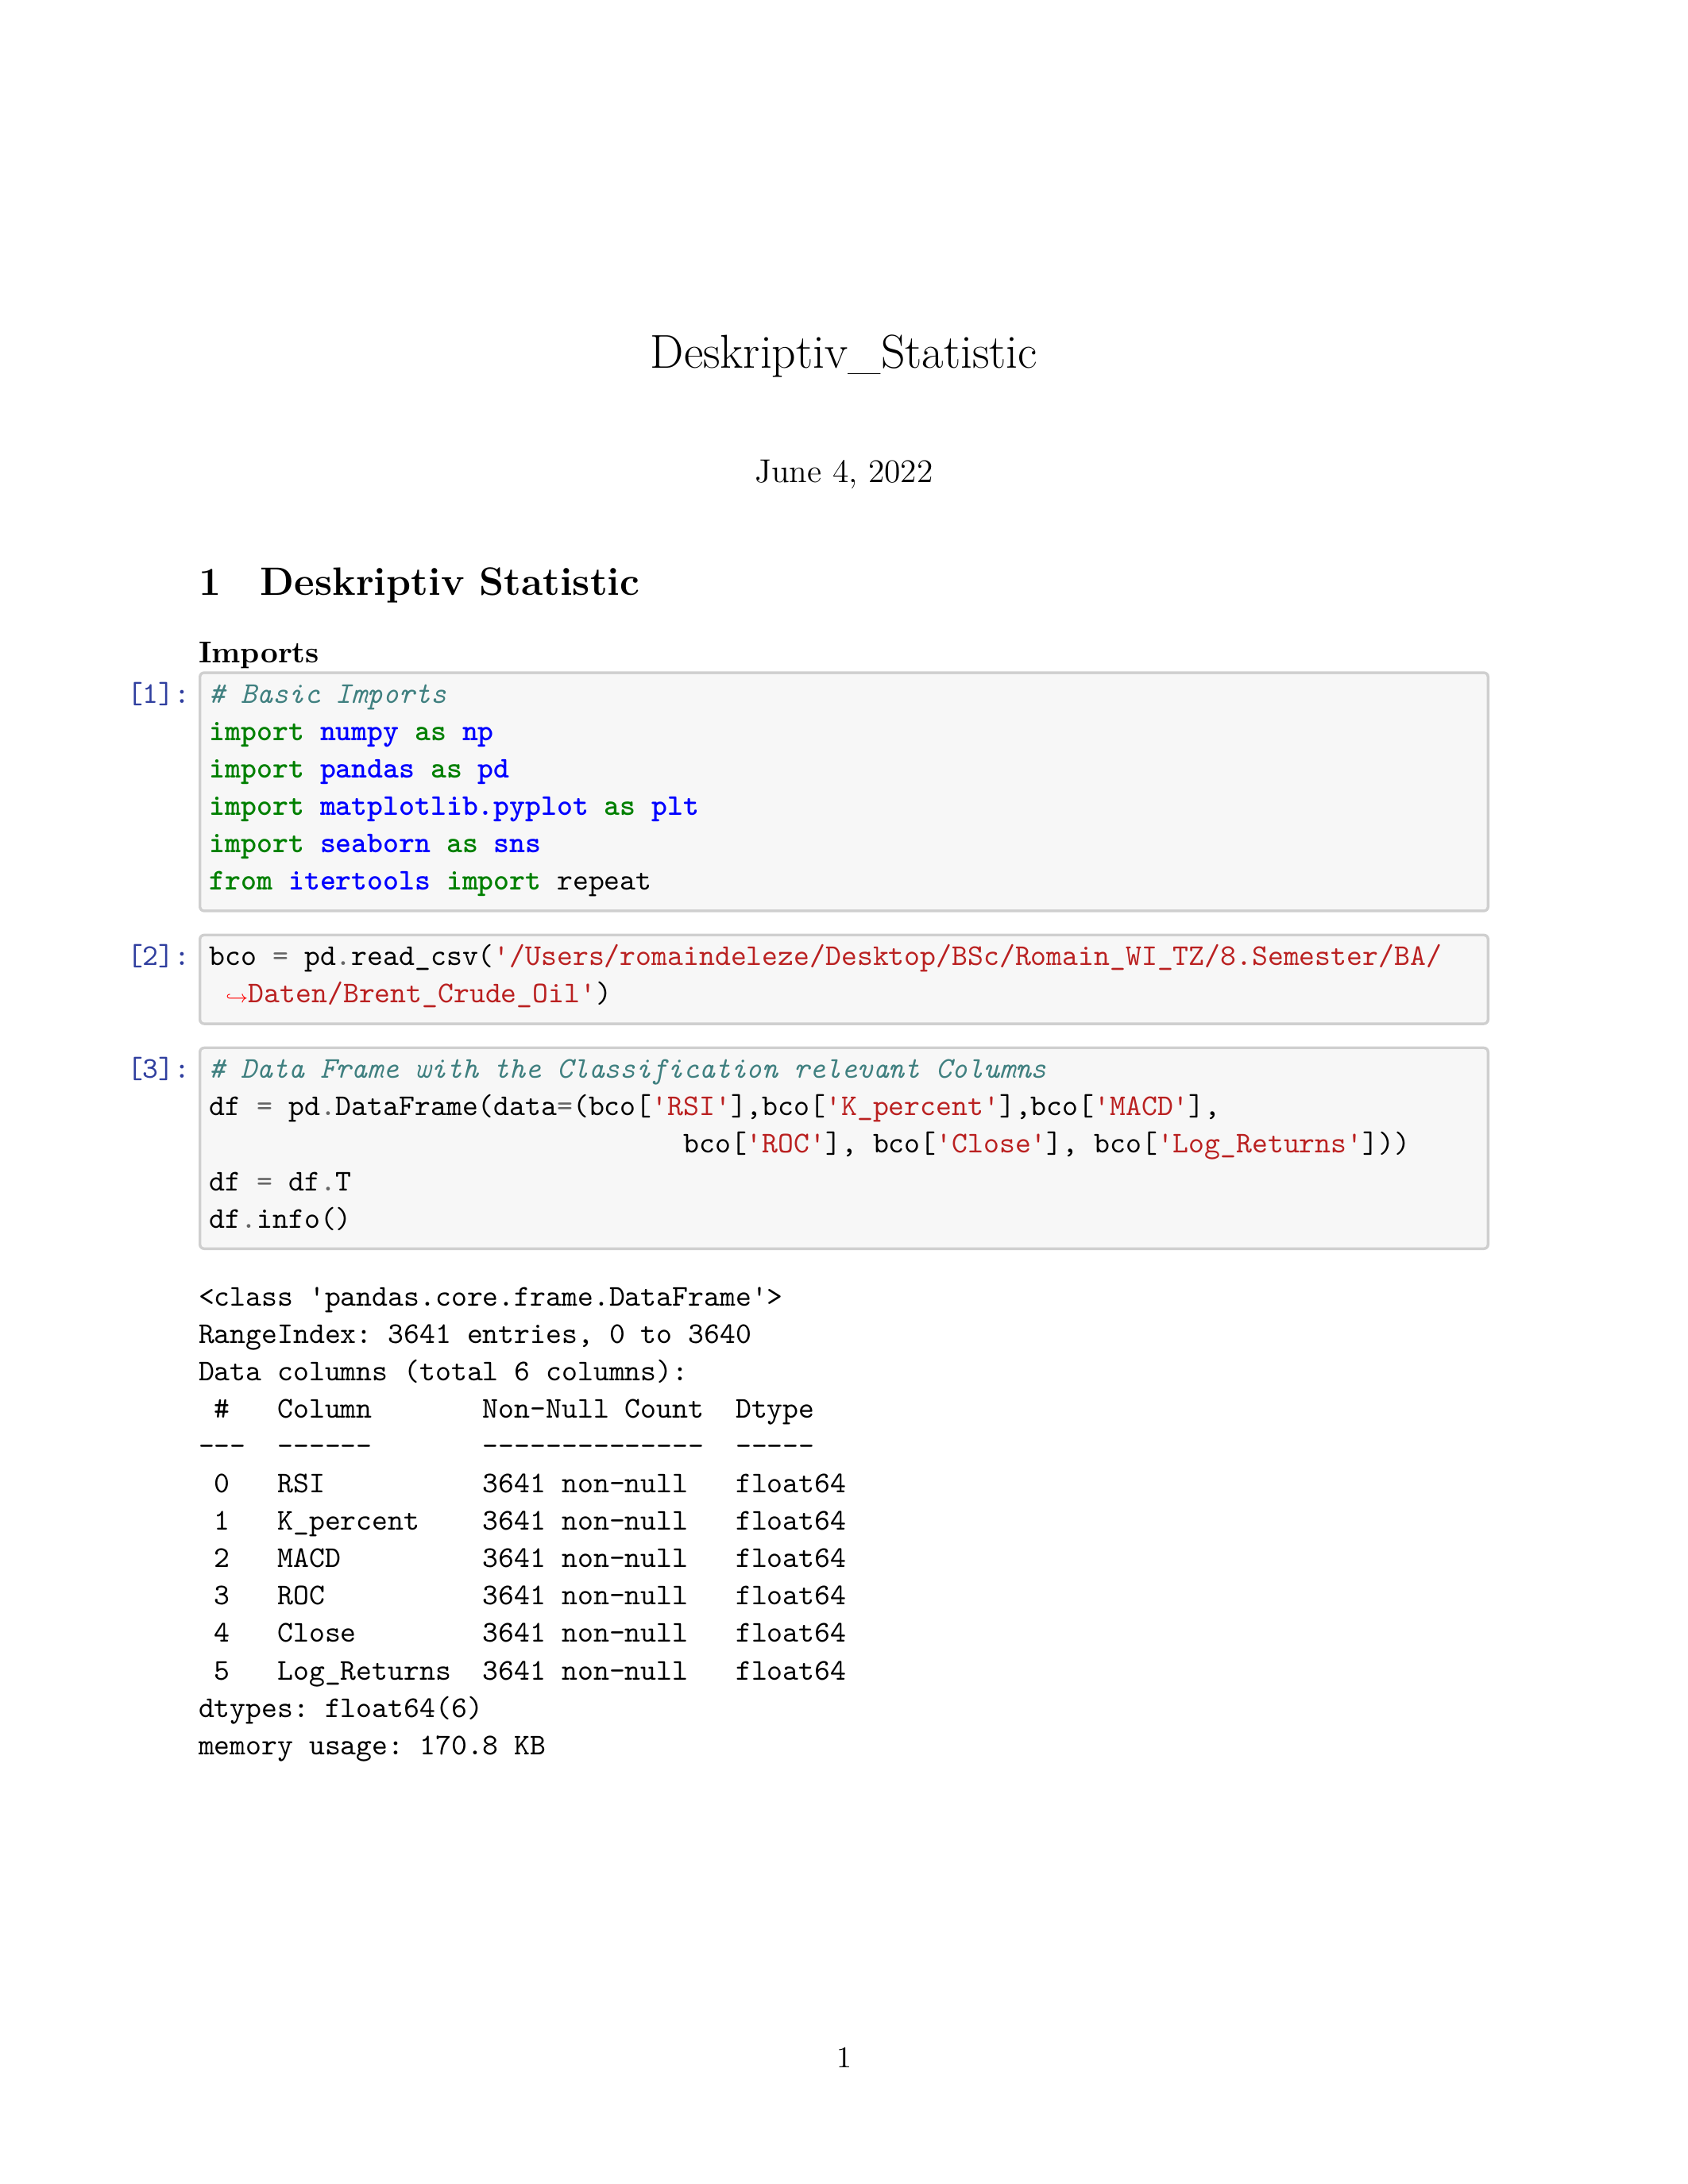}
\includepdf[pages=-]{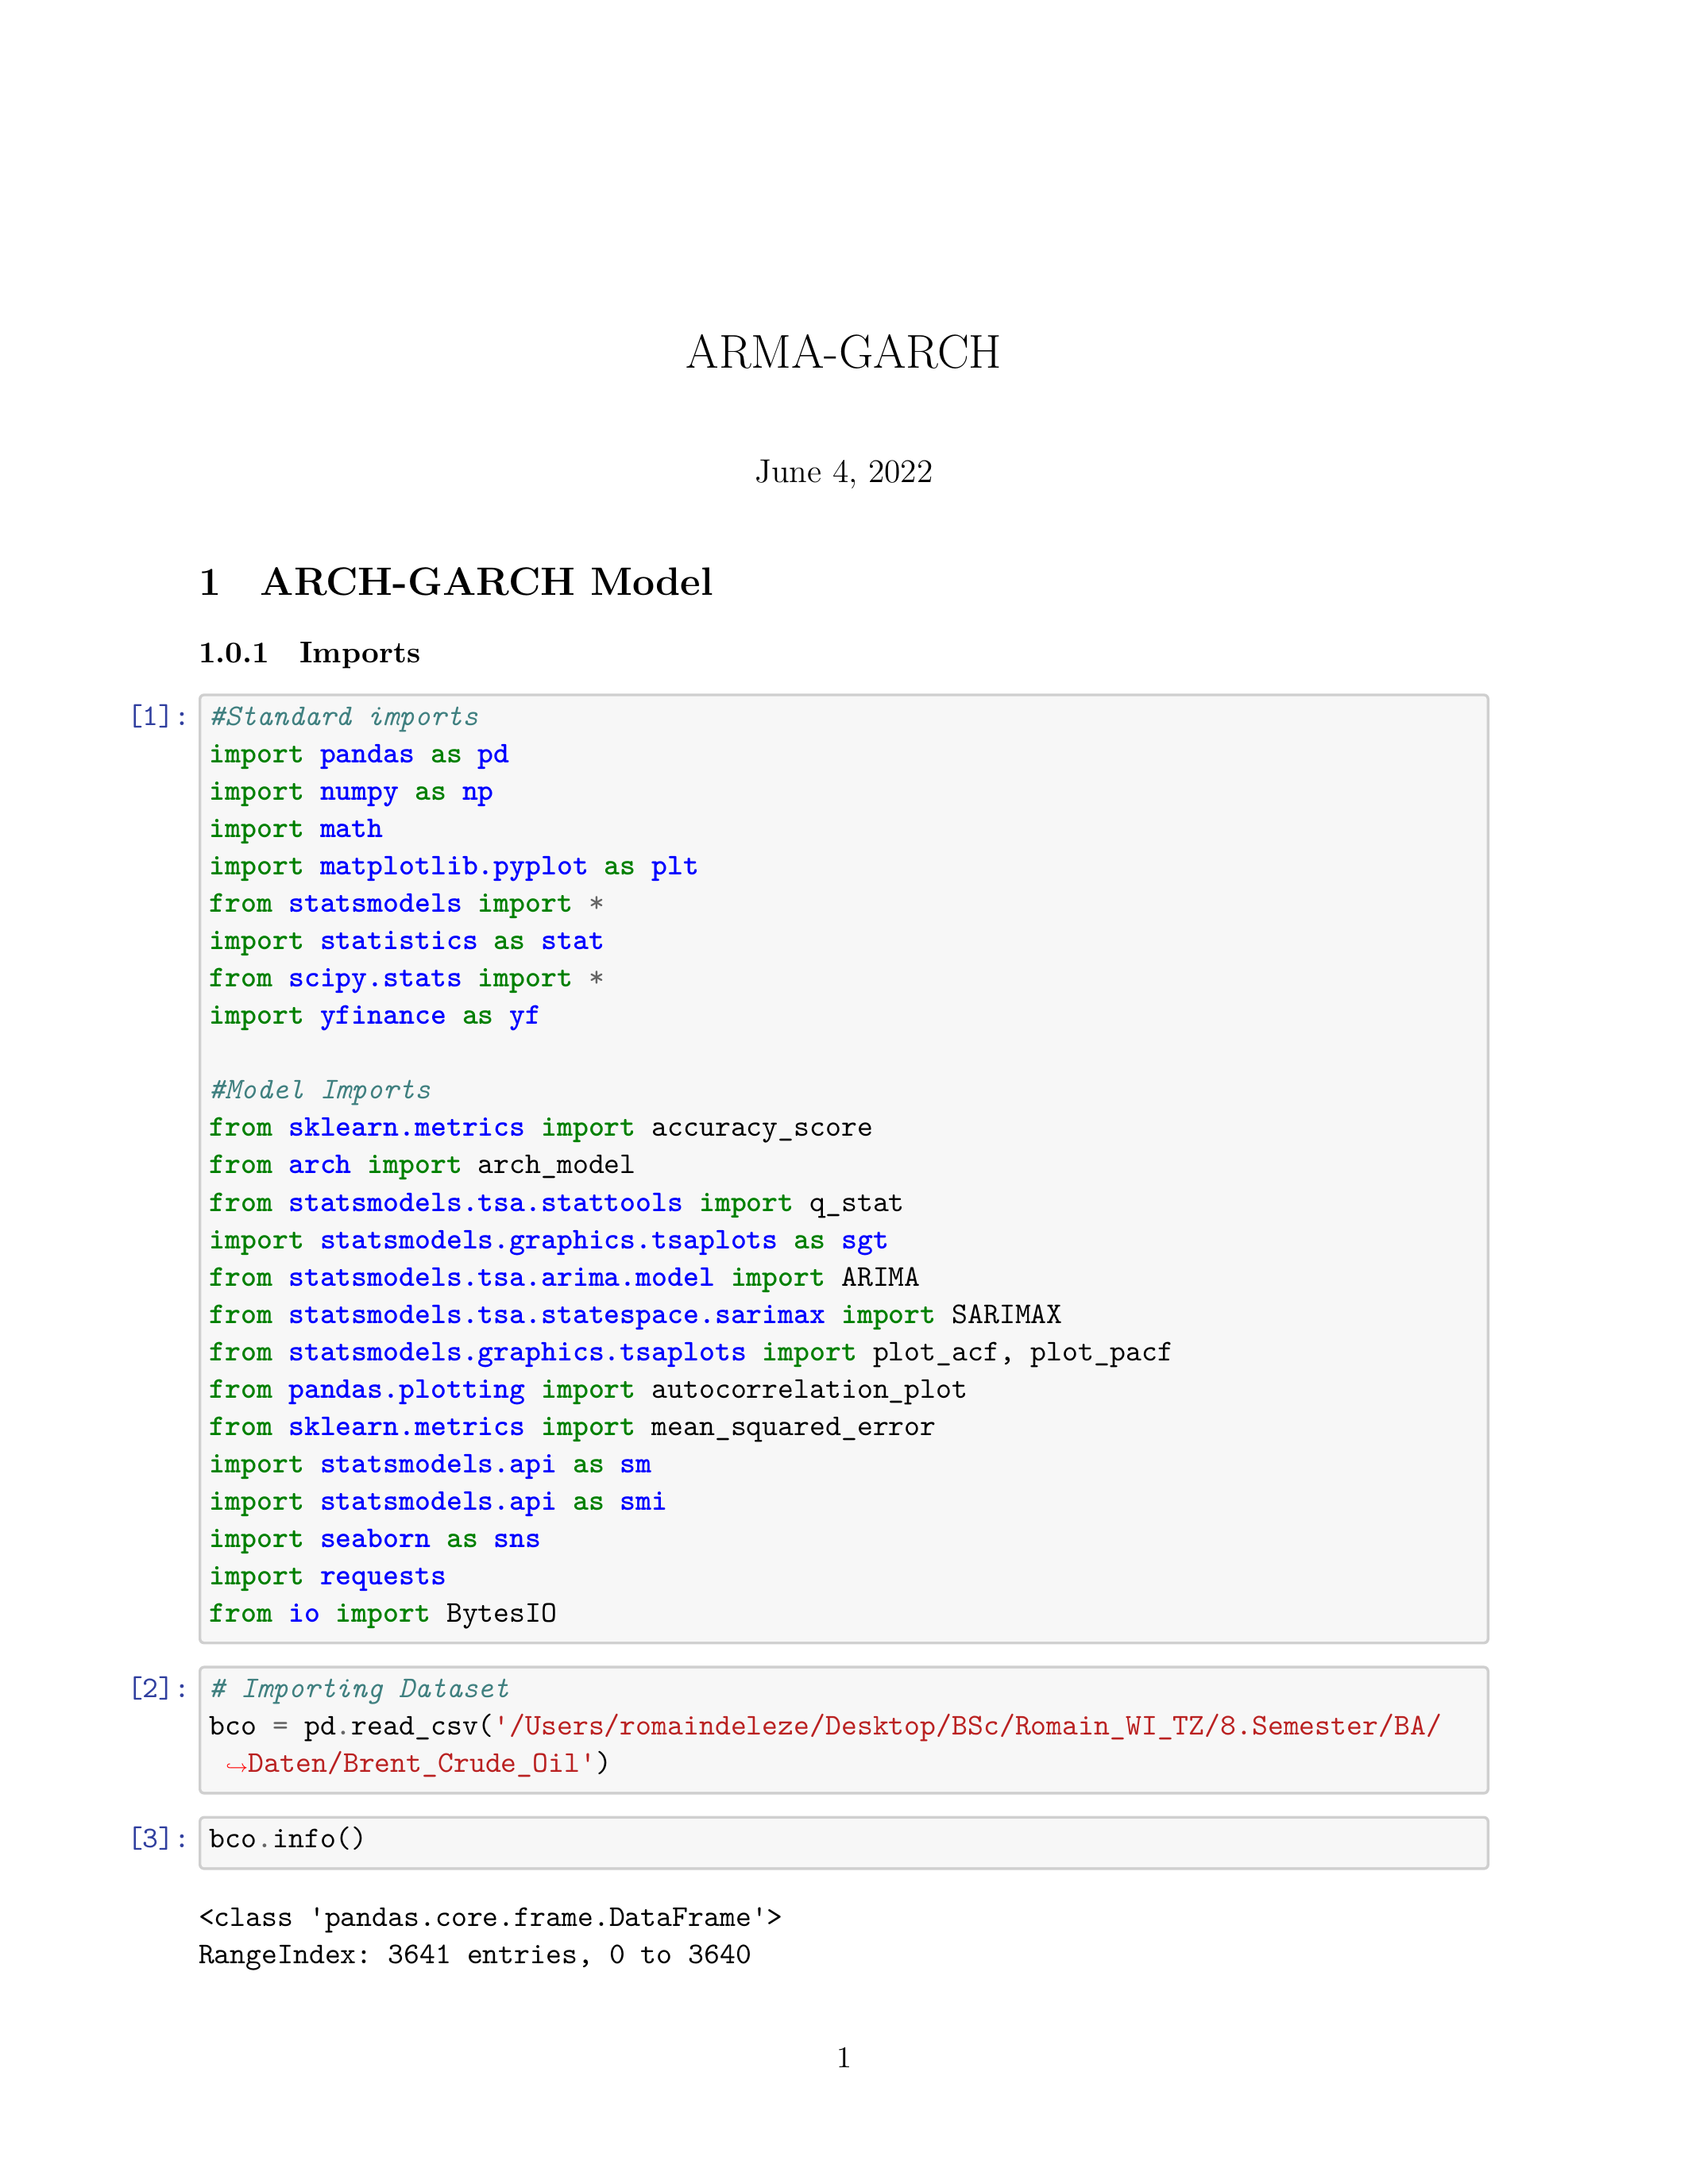}
\includepdf[pages=-]{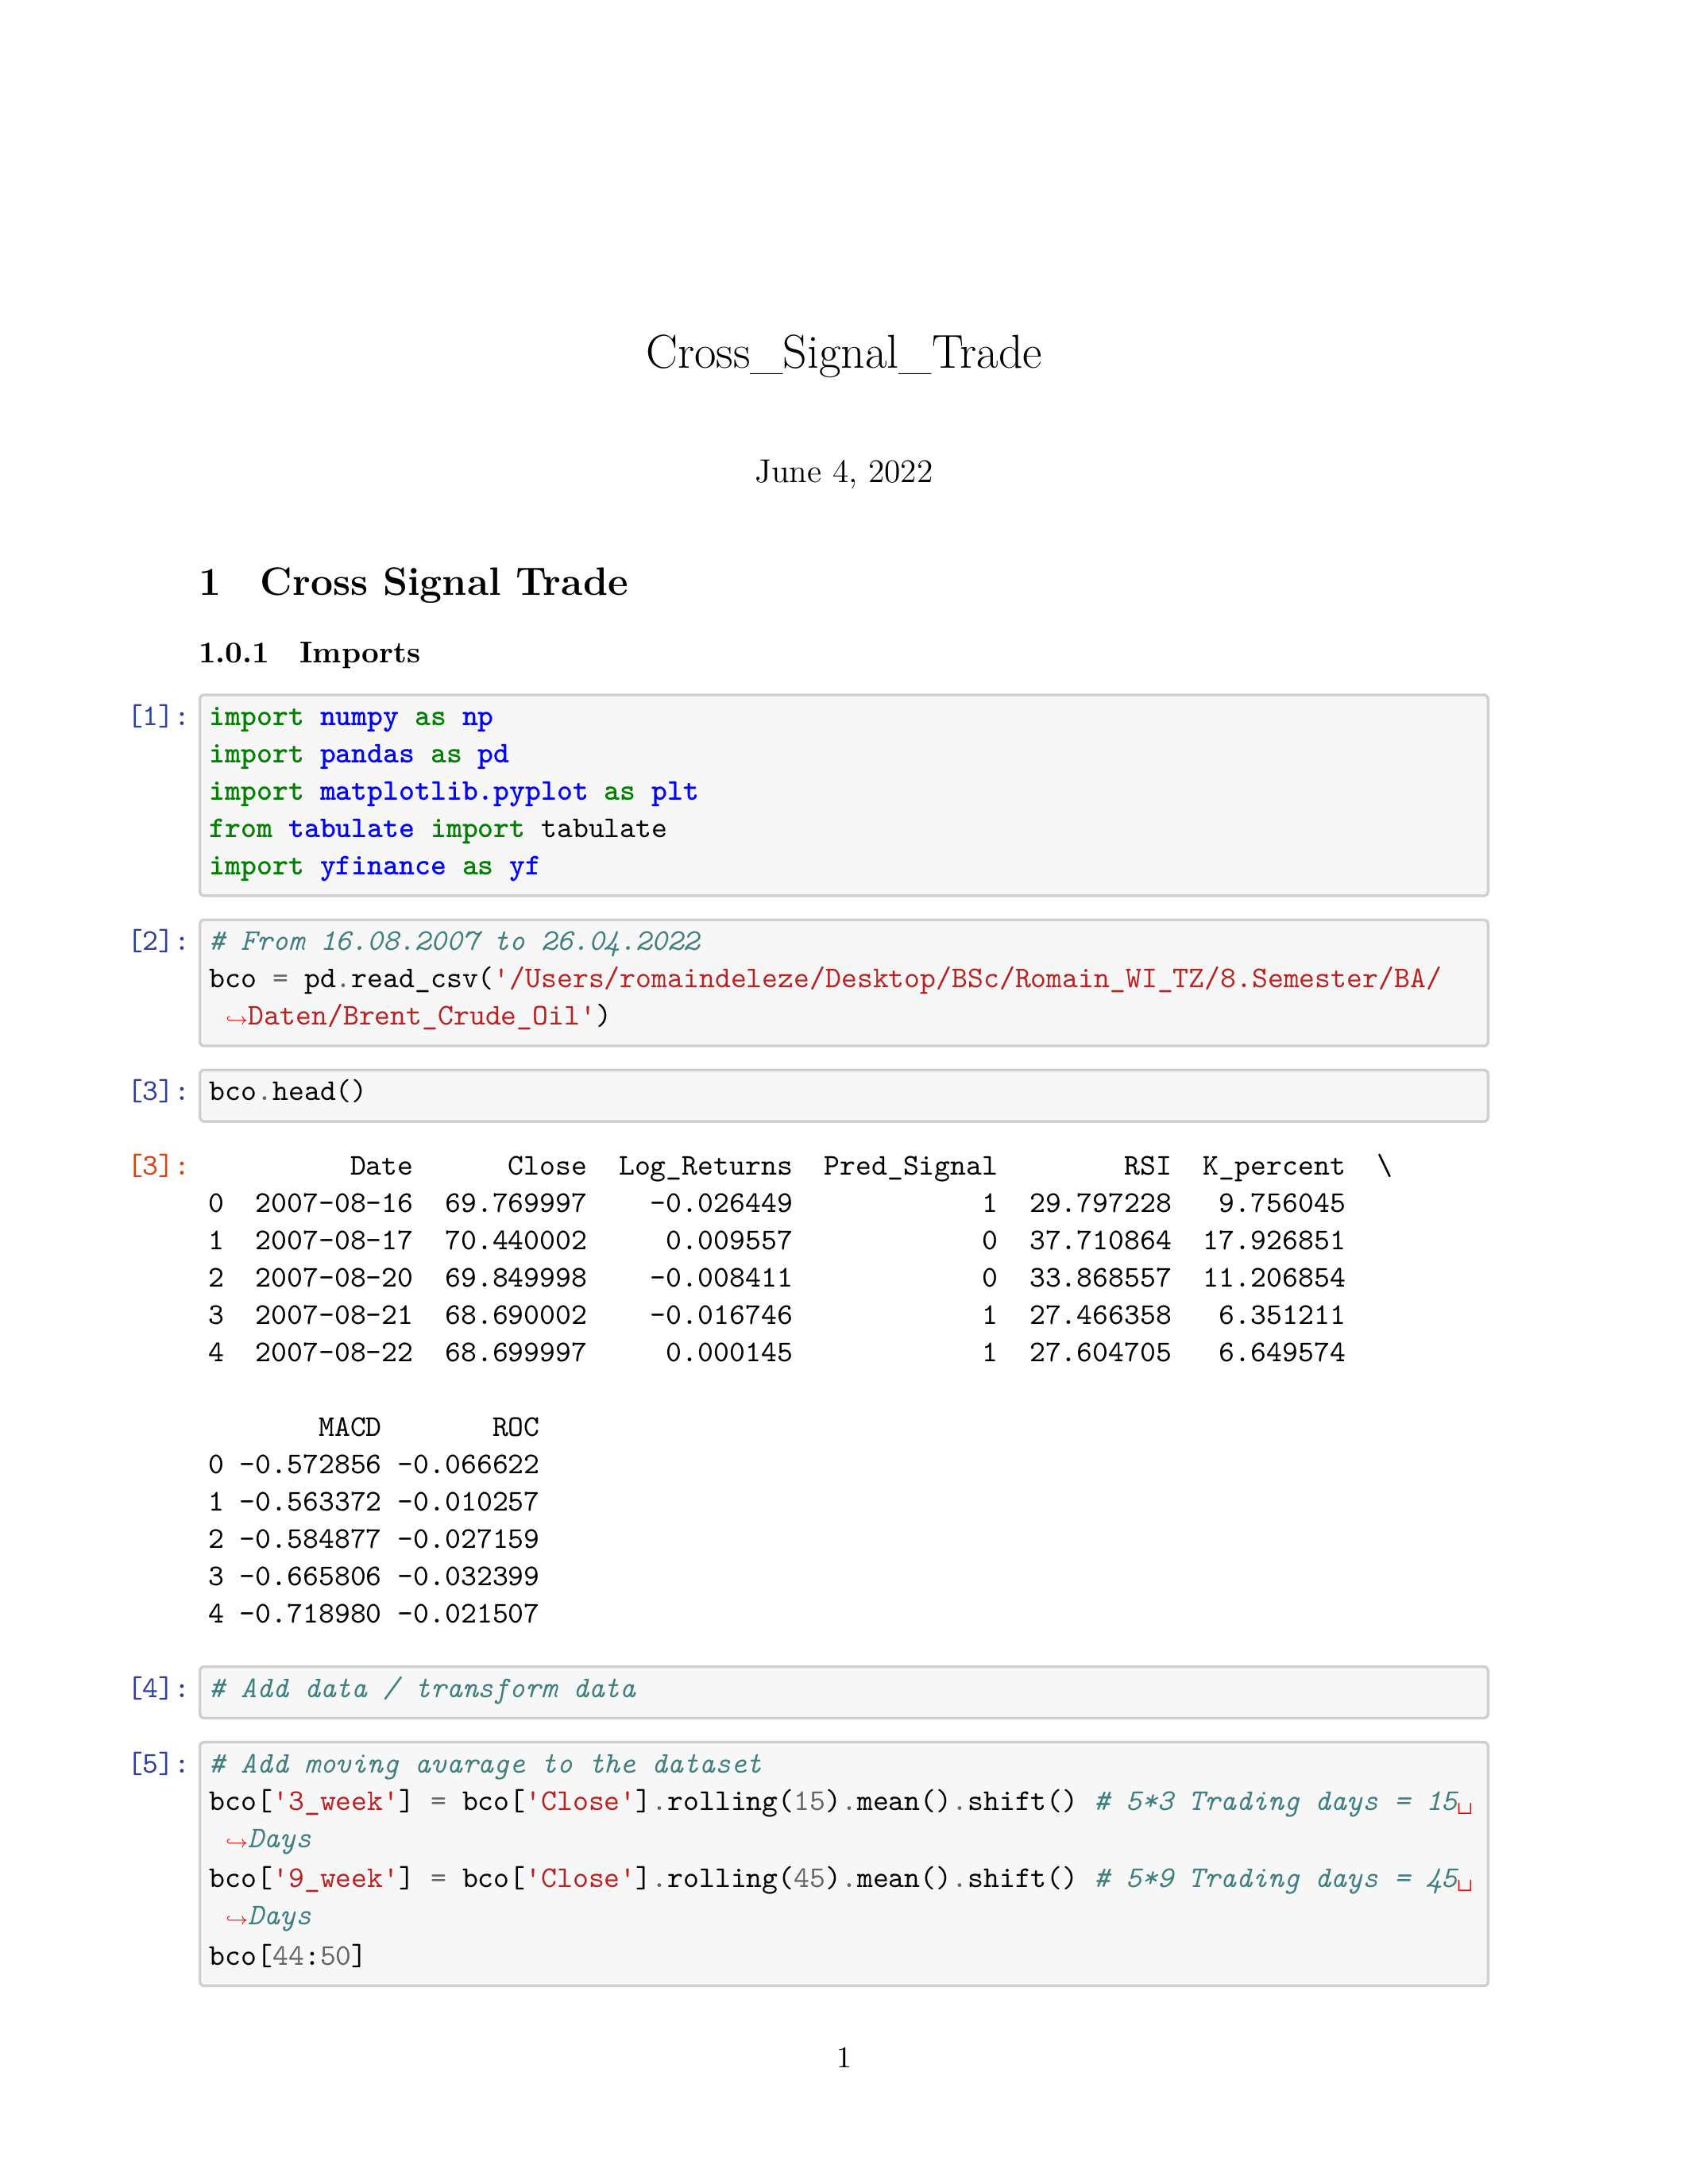}
\includepdf[pages=-]{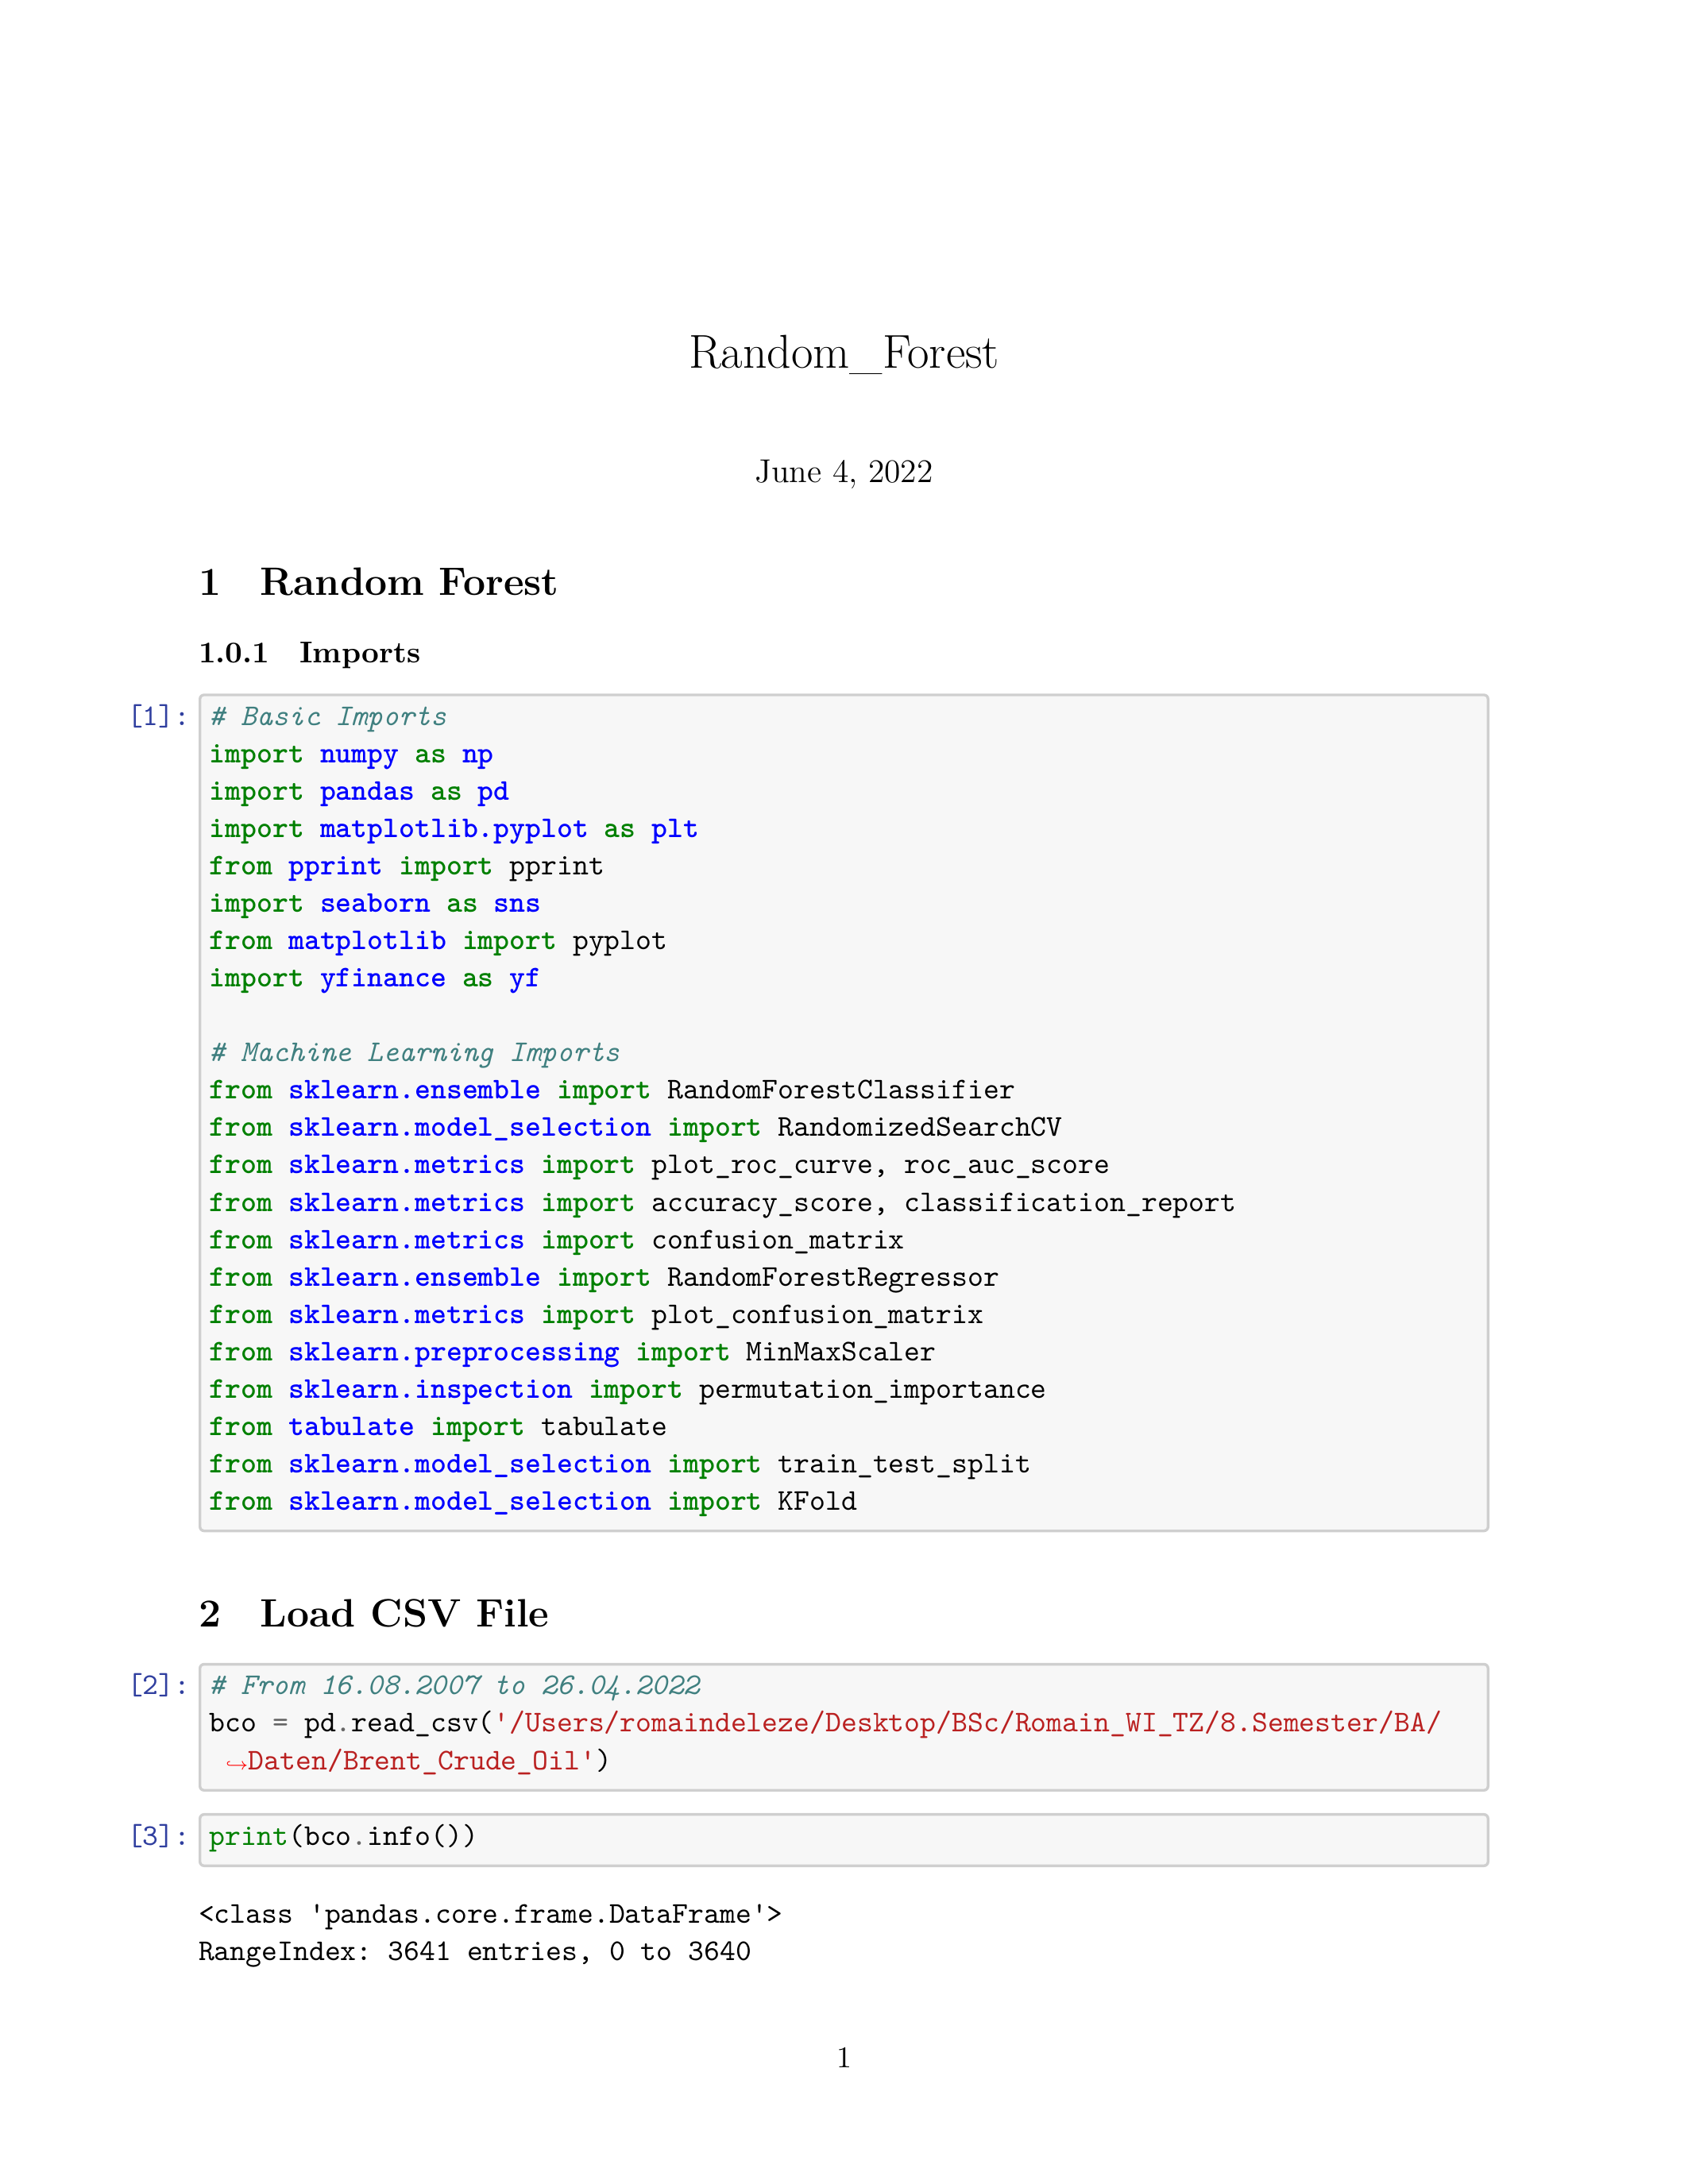}
\includepdf[pages=-]{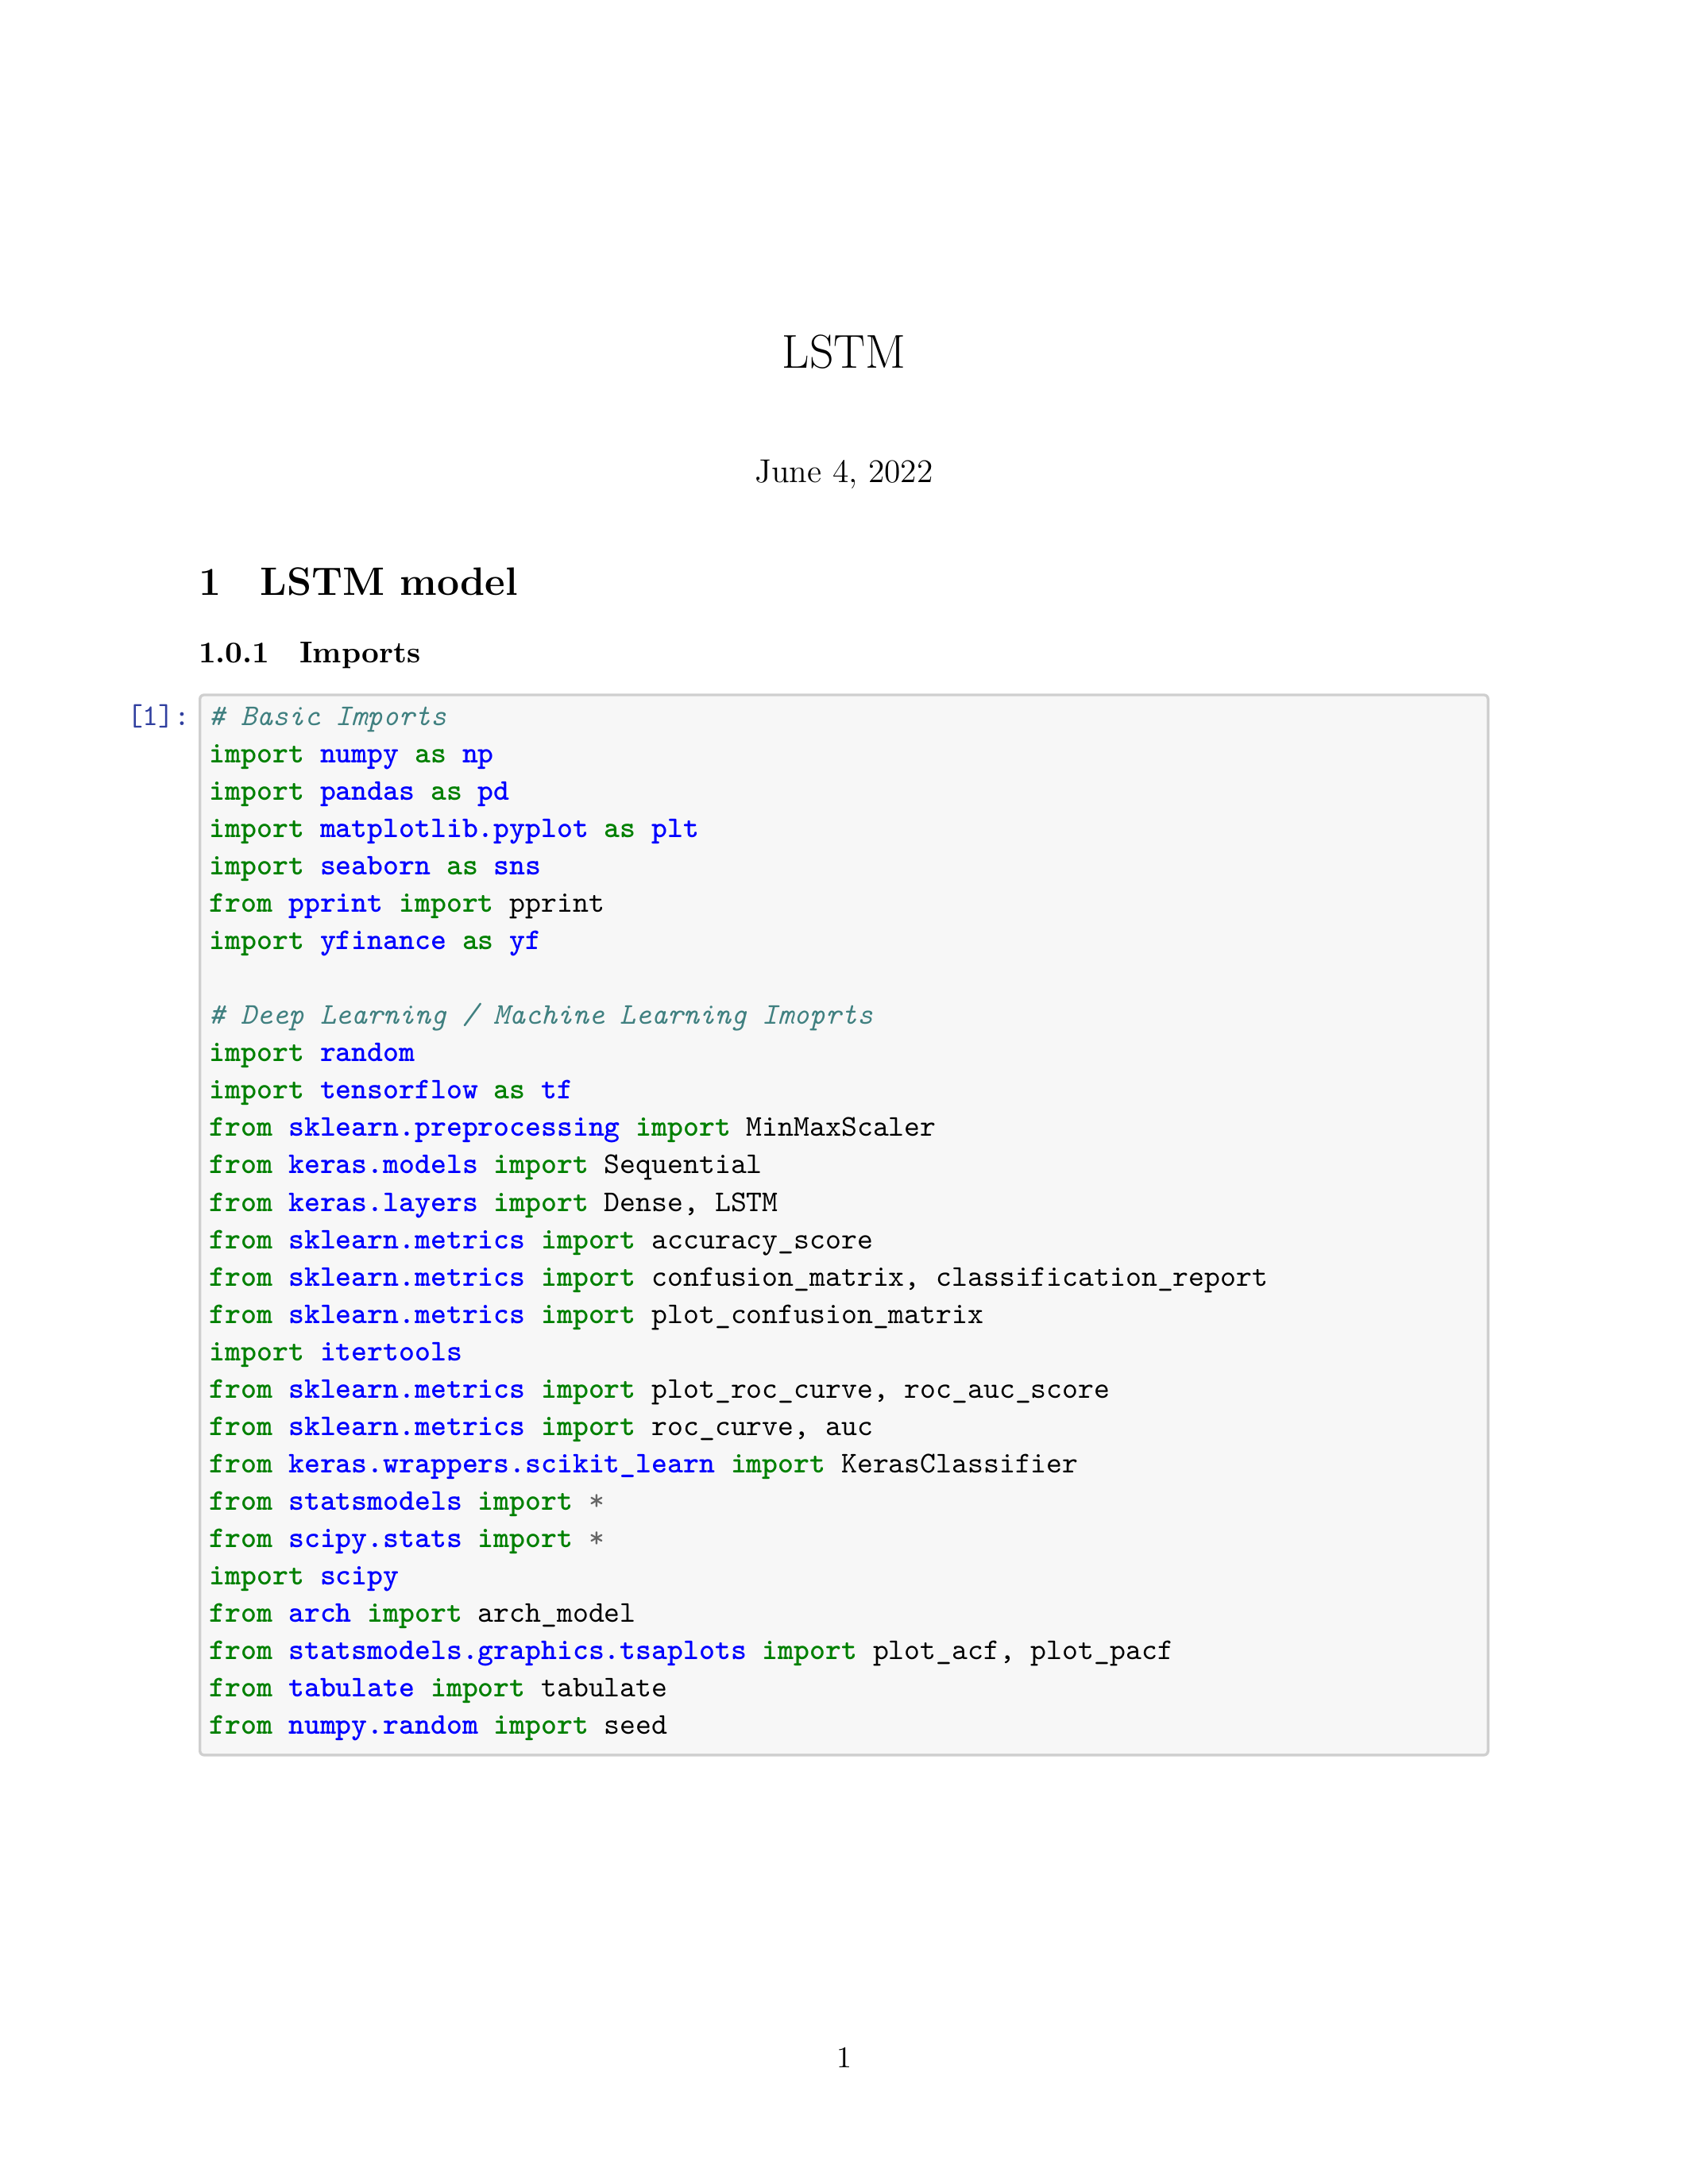}
\includepdf[pages=-]{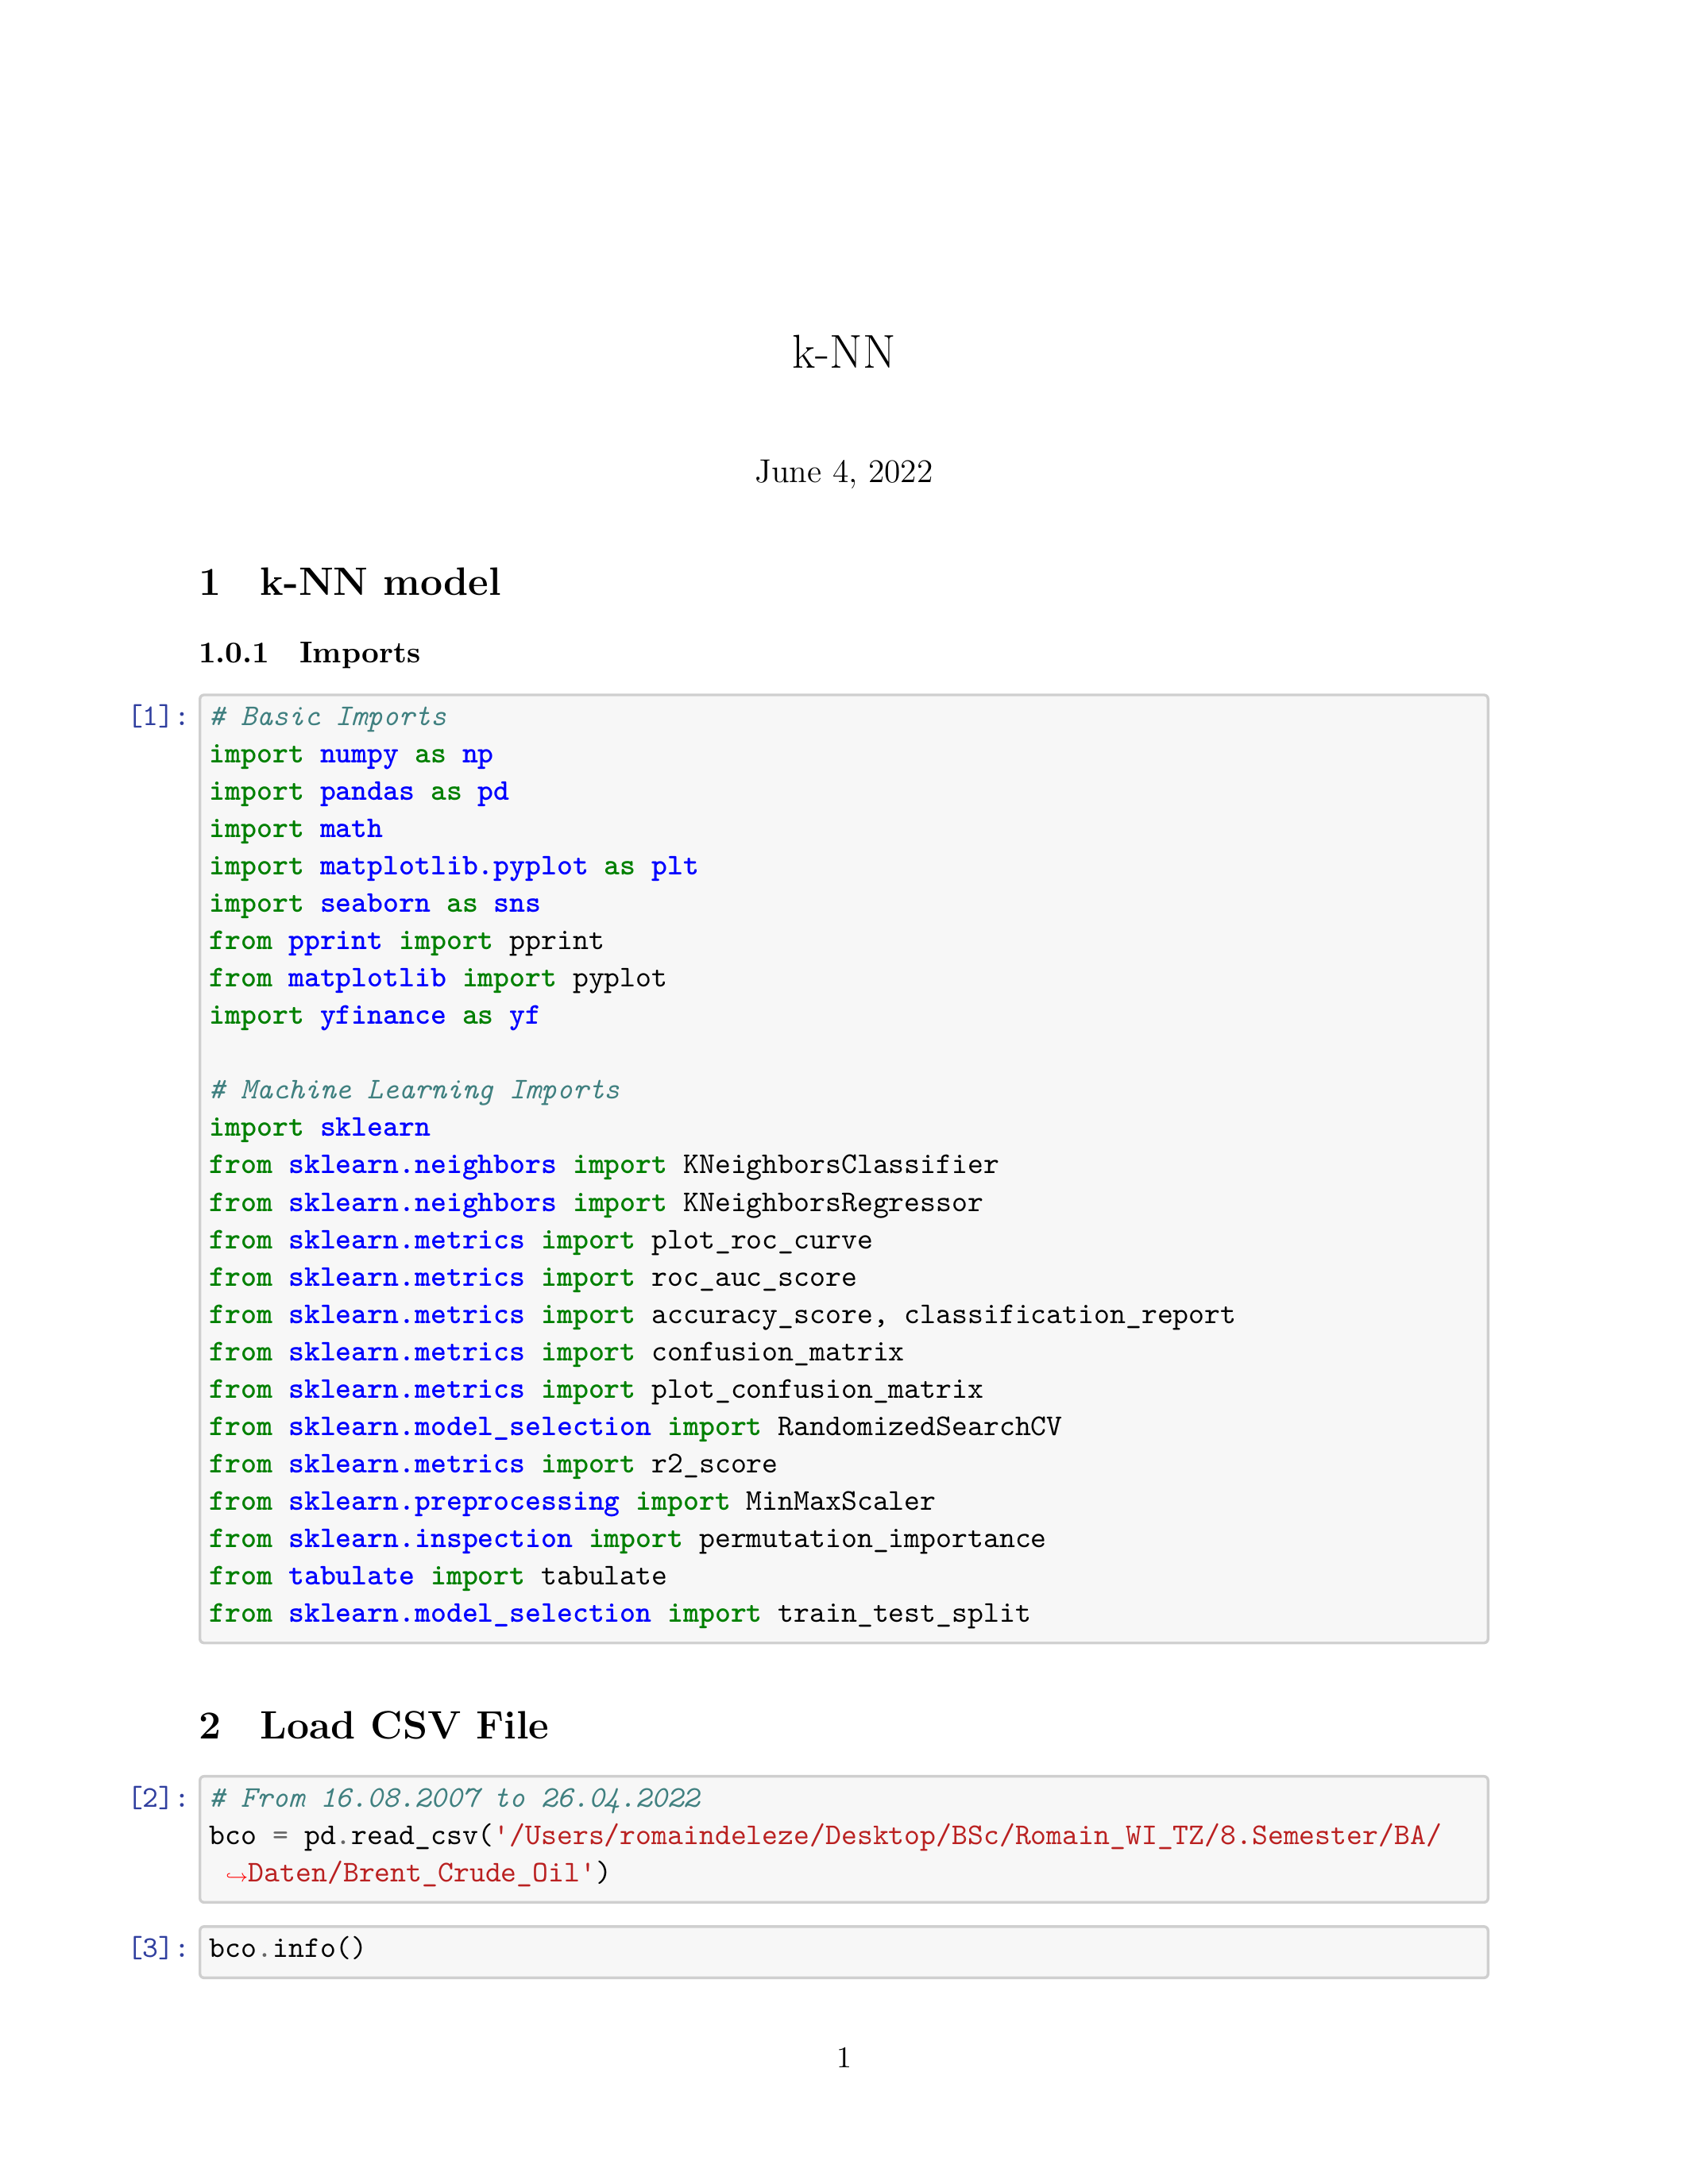}
\includepdf[pages=-]{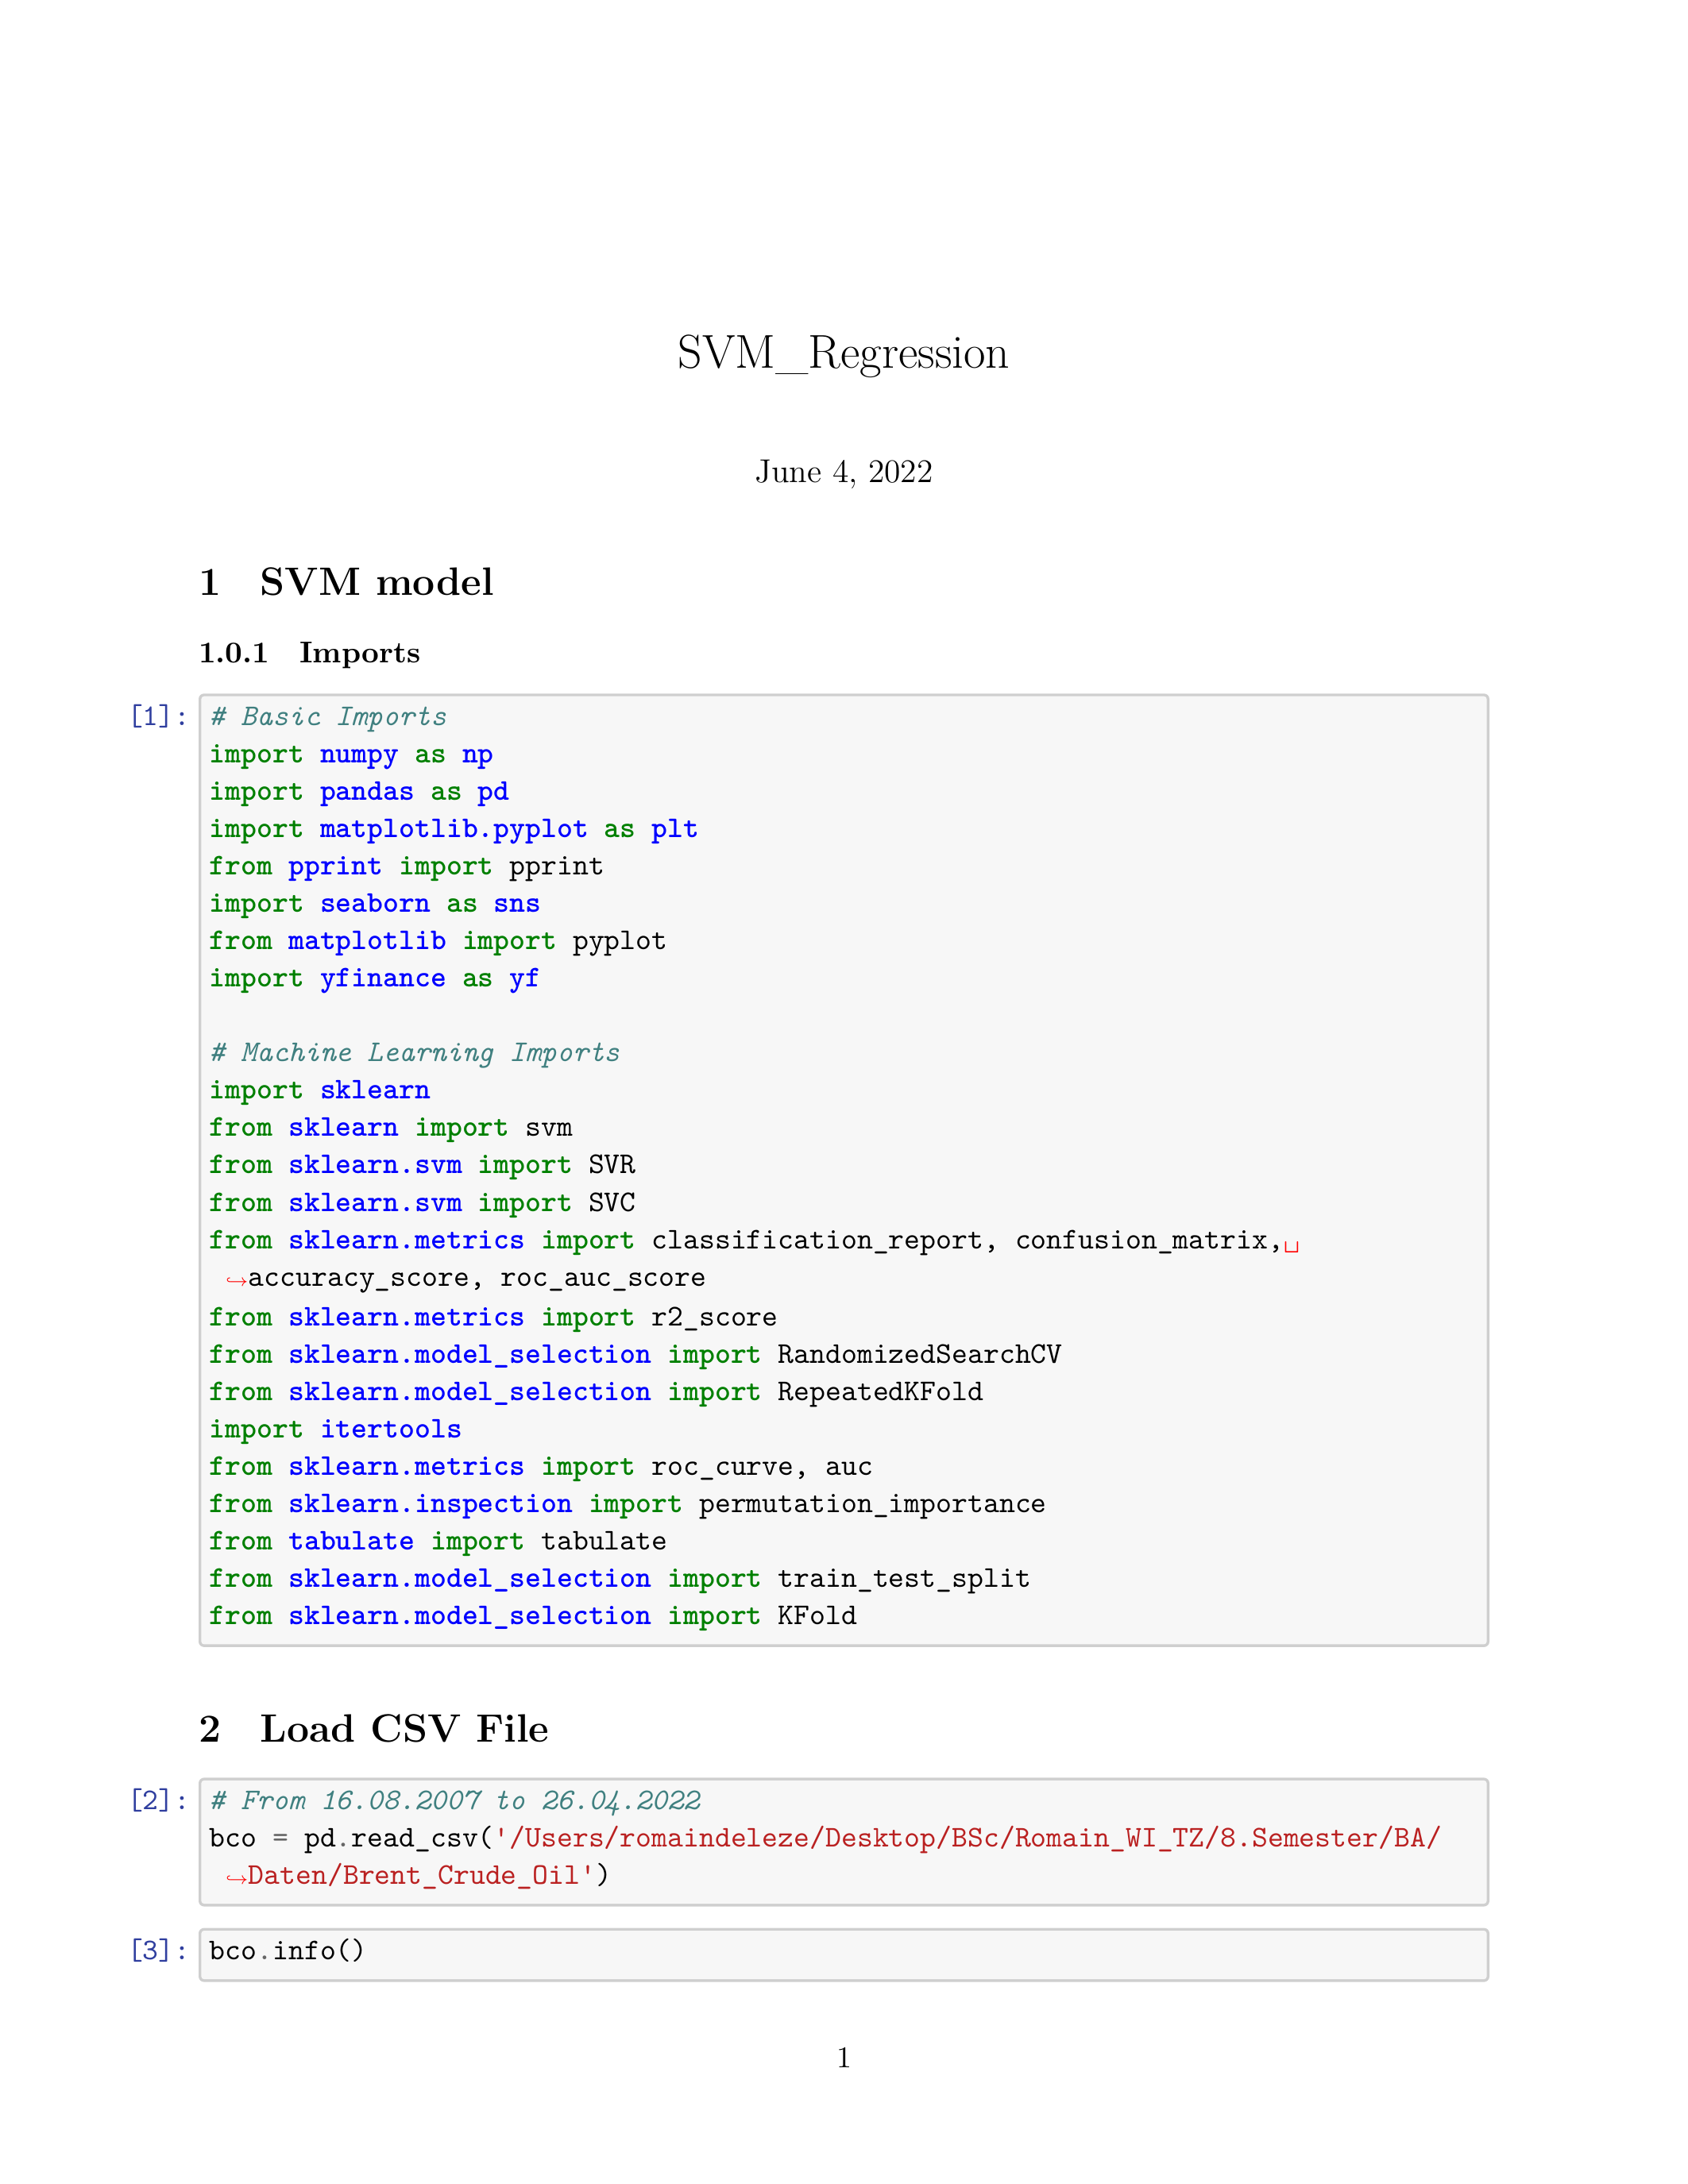}
